# Supplementary material for: Period-Amplitude Co-variation in Biomolecular Oscillators
Source: arXiv:1712.05606 ancillary file (2018-04-10)
Supplement: Supplementary file 1 [file Period-amplitude_co-variation_in_biomolecular_oscillators_Supplementary.pdf]

# Period-Amplitude Co-variation in Biomolecular Oscillators

Venkat Bokka [1], Abhishek Dey[2], Shaunak Sen[3]
Department of Electrical Engineering
Indian Institute of Technology Delhi
Hauz Khas, New Delhi 110016, INDIA
E-mail: venkatb@ee.iitd.ac.in[1], abhishek.dey@ee.iitd.ac.in[2], shaunak.sen@ee.iitd.ac.in[3]

# Contents


**1 Repressilator** **2**
1.1 Color Maps . . . 2
1.2 Co-variation of period and maximum amplitude . . . 3
1.3 Co-variation of period and amplitude metric ($M_p$) . . . 3

**2 Pentilator** **4**
2.1 Color Maps . . . 4
2.2 Co-variation of period and maximum amplitude . . . 5
2.3 Co-variation of period and amplitude metric ($M_p$) . . . 5

**3 Goodwin Oscillator** **6**
3.1 Color Maps . . . 7
3.2 Co-variation of period and maximum amplitude . . . 8
3.3 Co-variation of period and amplitude metric ($M_p$) . . . 8

**4 Van der Pol Oscillator** **9**
4.1 Color Maps . . . 9
4.2 Co-variation of period and maximum amplitude . . . 9
4.3 Co-variation of period and amplitude metric ($M_p$) . . . 10

**5 Fitzhugh-Nagumo oscillator** **11**
5.1 Color Maps . . . 11
5.2 Co-variation of period and maximum amplitude . . . 12
5.3 Co-variation of period and amplitude metric ($M_p$) . . . 12

**6 Frzilator** **13**
6.1 Color Maps . . . 13
6.2 Co-variation of period and maximum amplitude . . . 14
6.3 Co-variation of period and amplitude metric ($M_p$) . . . 14

**7 Cyanobacteria circadian oscillator** **15**
7.1 Color Maps . . . 16
7.2 Co-variation of period and maximum amplitude . . . 19
7.3 Co-variation of period and amplitude metric ($M_p$) . . . 20

**8 Metabolator** **21**
8.1 Color Maps . . . 22
8.2 Co-variation of period and maximum amplitude . . . 26
8.3 Co-variation of period and amplitude metric ($M_p$) . . . 27

**9 Mixed feedback oscillator** **28**
9.1 Color Maps . . . 28
9.2 Co-variation of period and maximum amplitude . . . 29
9.3 Co-variation of period and amplitude metric ($M_p$) . . . 29

**10 Meyer and Stryer model of calcium oscillations** **30**
10.1 Color Maps . . . 30
10.2 Co-variation of period and maximum amplitude . . . 32
10.3 Co-variation of period and amplitude metric ($M_p$) . . . 32

**11 Kim-Forger model** **33**
11.1 Color Maps . . . 34
11.2 Co-variation of period and maximum amplitude . . . 35
11.3 Co-variation of period and amplitude metric ($M_p$) . . . 35

# 1 Repressilator

The repressilator is a synthetic oscillatory network in which three proteins represses the other in a cyclic mode. The kinetics of the repressilator is given by first-order coupled differential equations for each combination of mRNA ($m_i$) and repressor-protein ($p_i$) concentrations. In total we have six states [1],

$$\begin{aligned} \dot{m}_i &= -k_m m_i + \frac{\gamma}{1 + k_b p_j^n} + \gamma_0, \\ \dot{p}_i &= -k_p p_i + \tau m_i, \end{aligned} \tag{1}$$

with $i = 1, 2, 3$ and $j = 3, 1, 2$.

Nominal Parameters: $n = 2$, $\gamma_0 = 0.0005$ nM s$^{-1}$, $\gamma = 0.5$ nM s$^{-1}$, $k_b = 1/1600$ nM, $k_m = 0.006$ s$^{-1}$, $k_p = 0.0012$ s$^{-1}$, $\tau = 0.12$ s$^{-1}$. Maximum amplitude of protein concentration is computed.

## 1.1 Color Maps

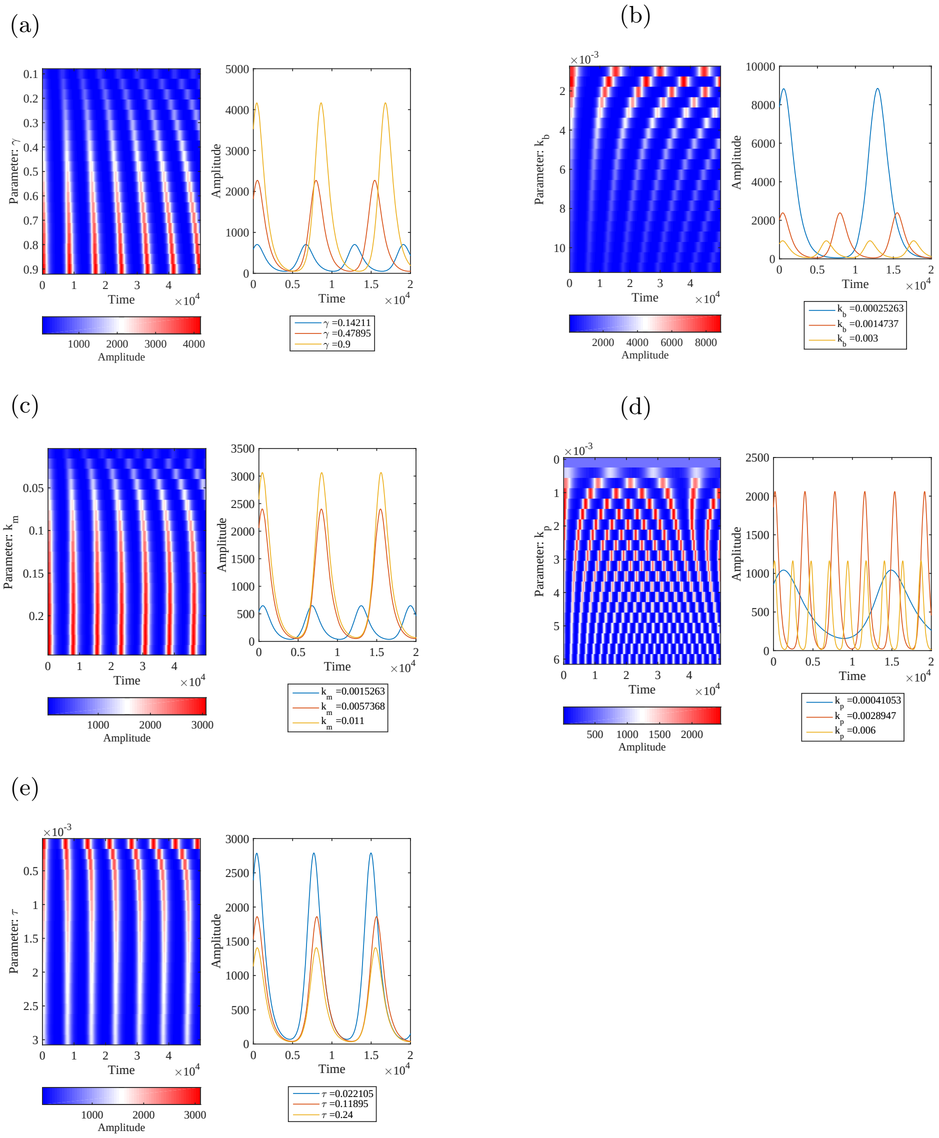


Figure 1-A : Repressilator. a) (left) Color-map with $\gamma = 0.05$ to 0.99. (right) Trajectories for different values of $\gamma$. b)(left) Color-map with $k_b = 0.0001$ to 0.0031. (right) Trajectories for different values of $k_b$. c) (left) Color-map with $k_m = 0.0006$ to 0.0115. (right) Trajectories for different values of $k_m$. d) (left) Color-map with $k_p = 0.0001$ to 0.0057. (right) Trajectories for different values of $k_p$. e) (left) Color-map with $\tau = 0.0116$ to 0.2306. (right) Trajectories for different values of $\tau$.

## 1.2 Co-variation of period and maximum amplitude

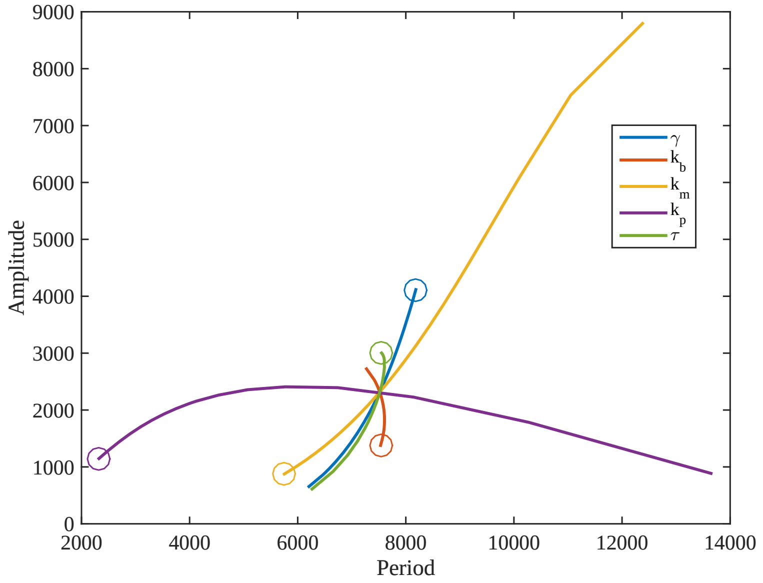


Figure 1-B : Repressilator. Co-variation of period and maximum amplitude of protein concentration. Circle shaped markers represent the largest value of the corresponding parameter. As parameter $\gamma$ increases, amplitude increases and period also increases. As parameter $k_b$ increases, the amplitude decreases and the period first increases then decreases. As parameter $k_m$ increases, the amplitude and period both decrease. As parameter $k_p$ increases, the amplitude first increases then decreases and the period decreases. As parameter $\tau$ increases, the amplitude increases and period increases.

## 1.3 Co-variation of period and amplitude metric ($M_p$)

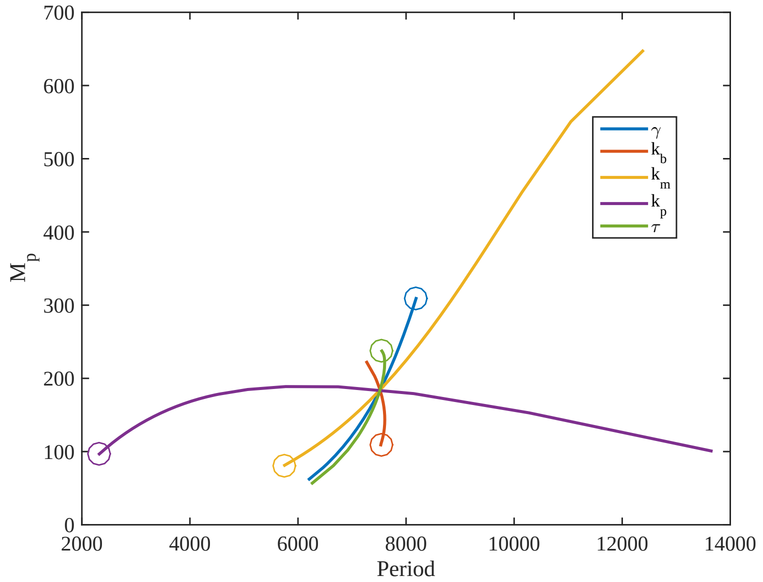


Figure 1-C : Repressilator. Co-variation of period and amplitude metric ($M_p$). Circle shaped markers represent the largest value of the corresponding parameter. As parameter $\gamma$ increases, $M_p$ and period increases. As parameter $k_b$ increases, $M_p$ decreases and the period increases. As parameter $k_m$ increases, $M_p$ decreases whereas the period decreases. As parameter $k_p$ increases, $M_p$ first increases then decrease and the period decreases continuously. As parameter $\tau$ increases, $M_p$ increases and period increases.

# 2 Pentilator

This is similar to the Repressilator model, only with five proteins instead of three. The mathematical model is [2],

$$\dot{m}_i = -k_m m_i + \frac{\gamma}{1 + k_b p_j^n} + \gamma_0, \qquad \dot{p}_i = -k_p p_i + \tau m_i, \tag{2}$$

with $i = 1, 2, 3, 4, 5$ and $j = 5, 1, 2, 3, 4$.

Nominal Parameters: $n = 2$, $\gamma_0 = 0.0005$ nM s$^{-1}$, $\gamma = 0.5$ nM s$^{-1}$, $k_b = 1/1600$ nM, $k_m = 0.006$ s$^{-1}$, $k_p = 0.0012$ s$^{-1}$, $\tau = 0.12$ s$^{-1}$. Maximum amplitude of protein concentration is computed.

## 2.1 Color Maps

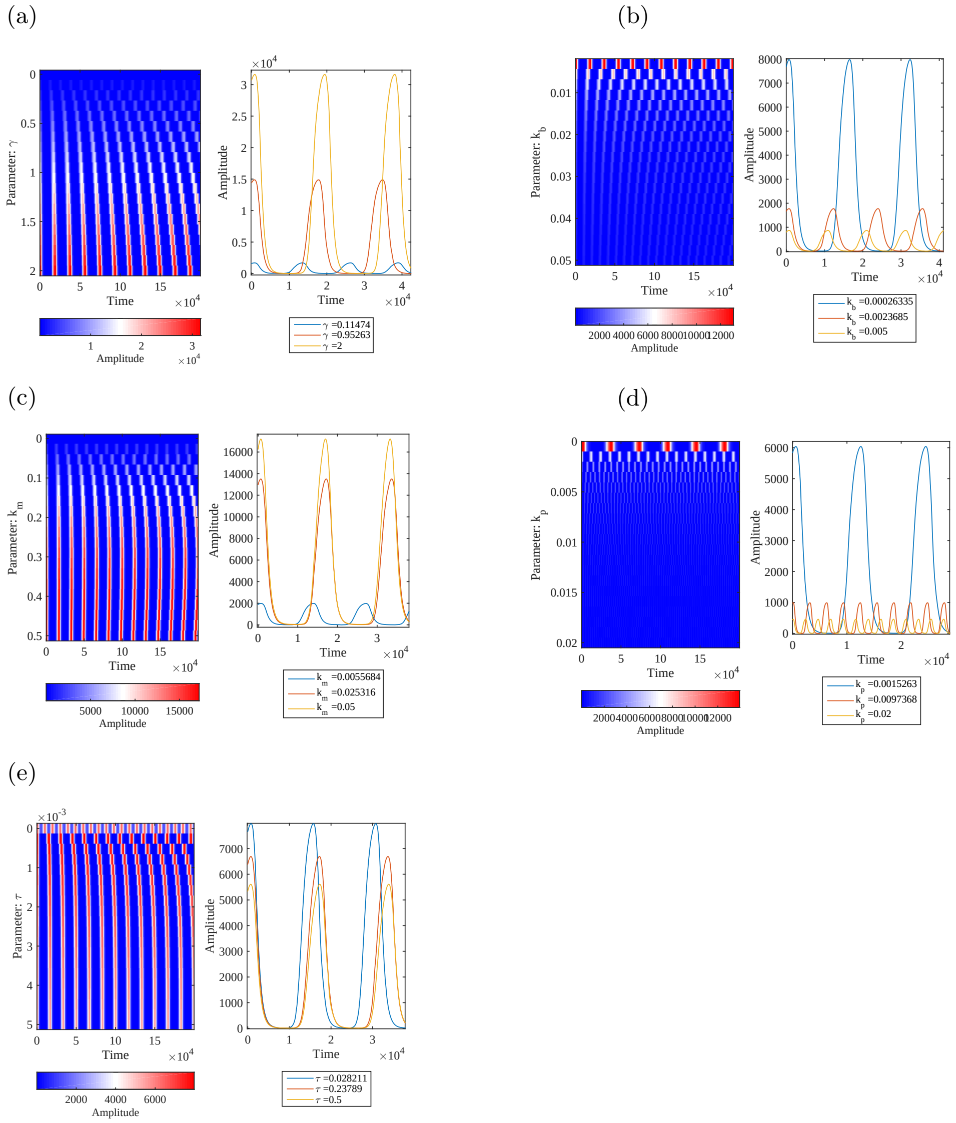


Figure 2-A : Pentilator. a) (left) Color-map with $\gamma = 0.01$ to 2. (right) Trajectories for different values of $\gamma$. b) (left) Color-map with $k_b = 0.0000002$ to 0.005. (right) Trajectories for different values of $k_b$. c) (left) Color-map with $k_m = 0.0031$ to 0.05. (right) Trajectories for different values of $k_m$. d) (left) Color-map with $k_p = 0.0005$ to 0.02. (right) Trajectories for different values of $k_p$. e) (left) Color-map with $\tau = 0.002$ to 0.5. (right) Trajectories for different values of $\tau$.

## 2.2 Co-variation of period and maximum amplitude

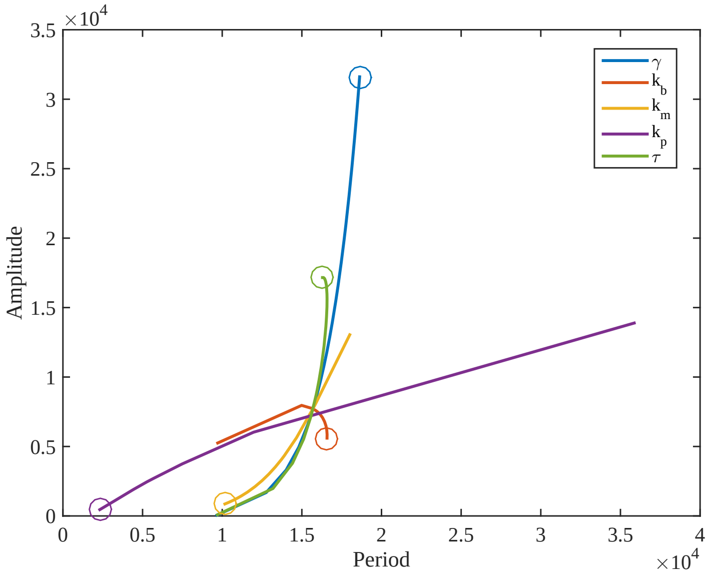


Figure 2-B : Pentilator. Co-variation of period and maximum amplitude of protein concentration. Circle shaped markers represent the largest value of the corresponding parameter. As parameter $\gamma$ increases, the amplitude increases and the period increases. As parameter $k_b$ increases, the amplitude first increases and then decreases while the period increases. As parameter $k_m$ increases, the amplitude decreases and the period decreases As parameter $k_p$ increases, the amplitude decreases and the period decreases. As parameter $\tau$ increases, the amplitude increases and the period increases.

## 2.3 Co-variation of period and amplitude metric ($M_p$)

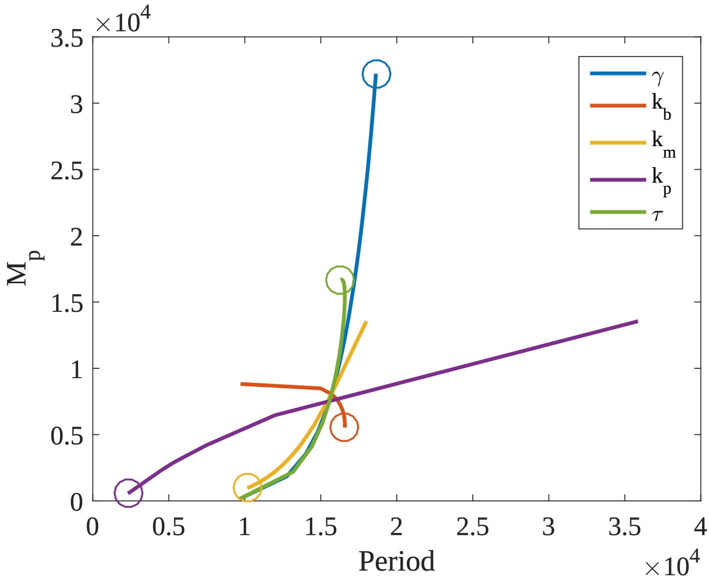


Figure 2-C : Pentilator. Co-variation of period and amplitude metric ($M_p$). Circle shaped markers represent the largest value of the corresponding parameter. As parameter $\gamma$ increases, $M_1$ and $M_p$ increases and the period increases. As parameter $k_b$ increases, $M_p$ decreases and the period increases in both cases. As parameter $k_m$ increases, $M_p$ decreases and the period decreases As parameter $k_p$ increases, $M_p$ decreases and period decreases. As parameter $\tau$ increases, $M_p$ increases and the period increases

## 3 Goodwin Oscillator

Goodwin oscillator is a three state model where protein y is produced by mRNA x and the transcriptional inhibitor z is activated by y with the production of x by z [3],

$$\begin{aligned} \dot{x} &= \frac{k_1}{1 + (\frac{z}{k_7})^n} - k_4 x, \\ \dot{y} &= k_2 x - k_5 y, \\ \dot{z} &= k_3 y - k_6 z, \end{aligned} \tag{3}$$

with $n = 15$, $k_1 = k_2 = k_3 = 1$, $k_4 = 0.16$, $k_5 = 0.29$, $k_6 = 0.3$ and $k_7 = 1$. Maximum amplitude of protein $y$ is computed.

## 3.1 Color Maps

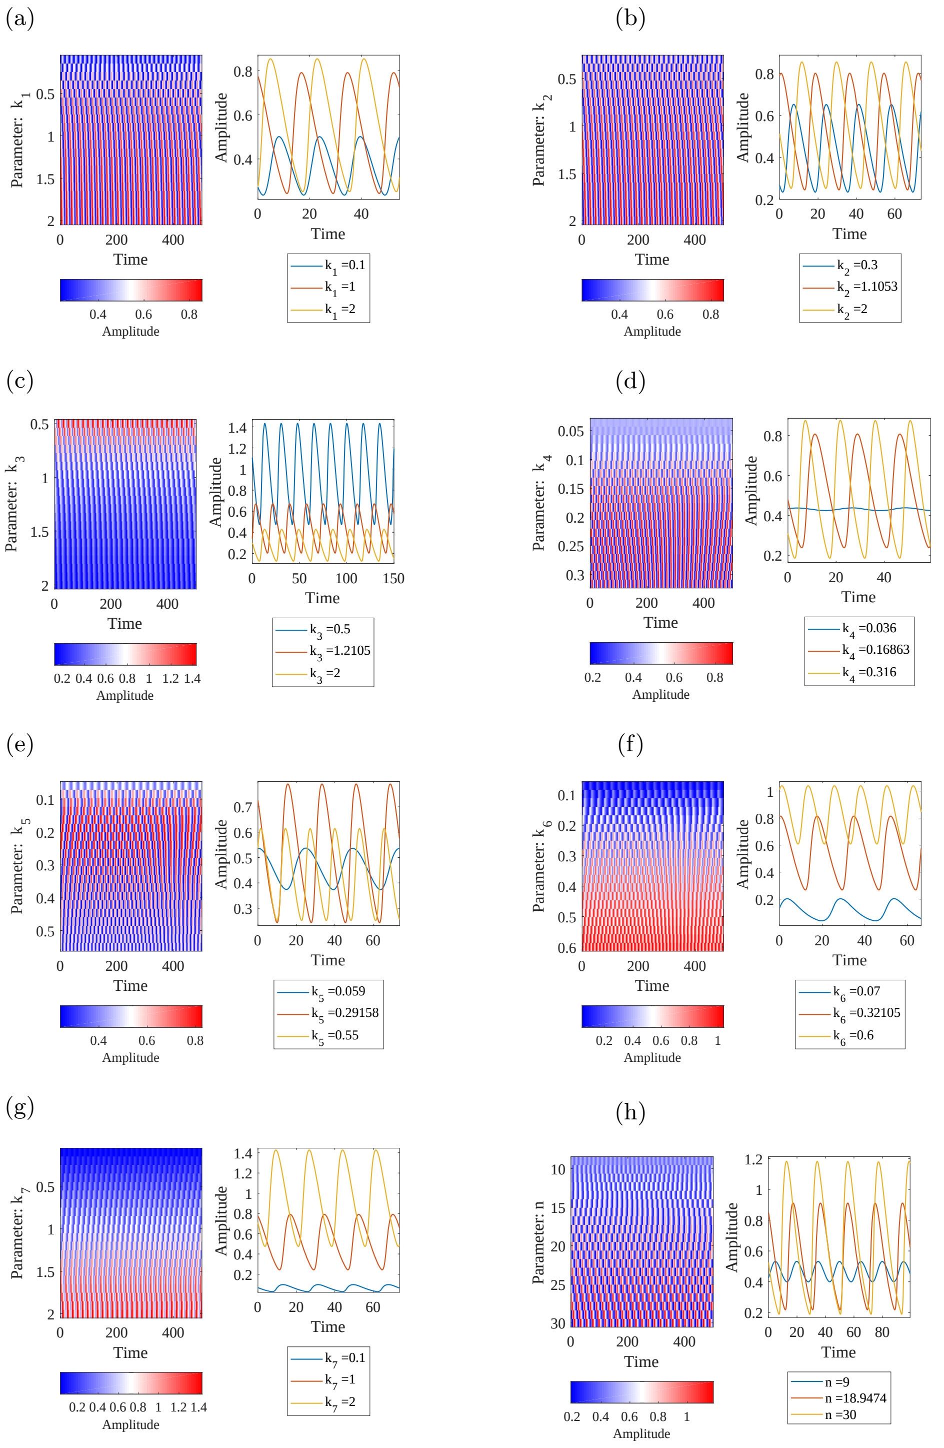


Figure 3-A : Goodwin Oscillator. a) (left) Color-map with $k_1 = 0.1$ to 2. (right) Trajectories for different values of $k_1$. b) (left) Color-map with $k_2 = 0.3$ to 2. (right) Trajectories for different values of $k_2$. c) (left) Color-map with $k_3 = 0.5$ to 2. (right) Trajectories for different values of $k_3$. d) (left) Color-map with $k_4 = 0.036$ to 0.316. (right) Trajectories for different values of $k_4$. e) (left) Color-map with $k_5 = 0.049$ to 0.579. (right) Trajectories for different values of $k_5$. f) (left) Color-map with $k_6 = 0.3$ to 0.6. (right) Trajectories for different values of $k_6$.g) (left) Color-map with $k_7 = 0.1$ to 2. (right) Trajectories for different values of $k_7$. h) (left) Color-map with $n = 9$ to 30. (right) Trajectories for different values of $n$.

## 3.2 Co-variation of period and maximum amplitude

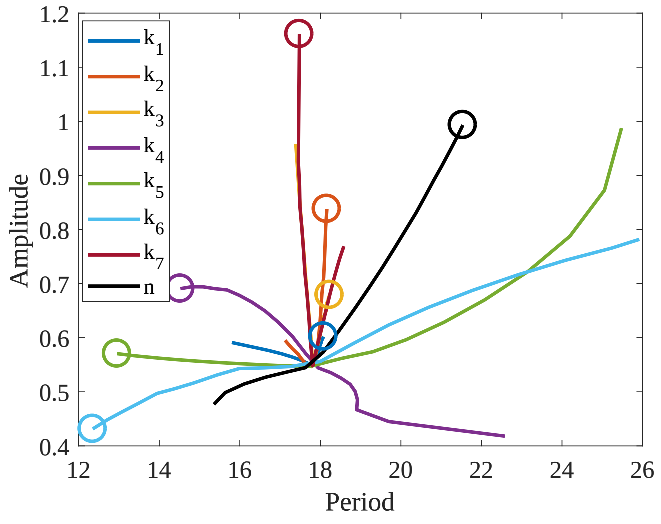


Figure 3-B : Goodwin Oscillator. Co-variation of period and maximum amplitude. Circle shaped markers represent the largest value of the corresponding parameter. As parameter $k_1$ increases, the amplitude first decreases then increases and the period slightly increases. As parameter $k_2$ increases, the amplitude increases and the period does not change significantly. As parameter $k_3$ increases, the amplitude first increases then decreases and the period does not change significantly. As parameter $k_4$ increases, the amplitude increases and the period decreases. As parameter $k_5$ increases, the amplitude decreases and the period decreases. As parameter $k_6$ increases, the amplitude decreases and the period decreases. As parameter $k_7$ increases, the amplitude first decreases then increases and the period does not change significantly. As parameter $n$ increases, the amplitude and the period increases.

## 3.3 Co-variation of period and amplitude metric ($M_p$)

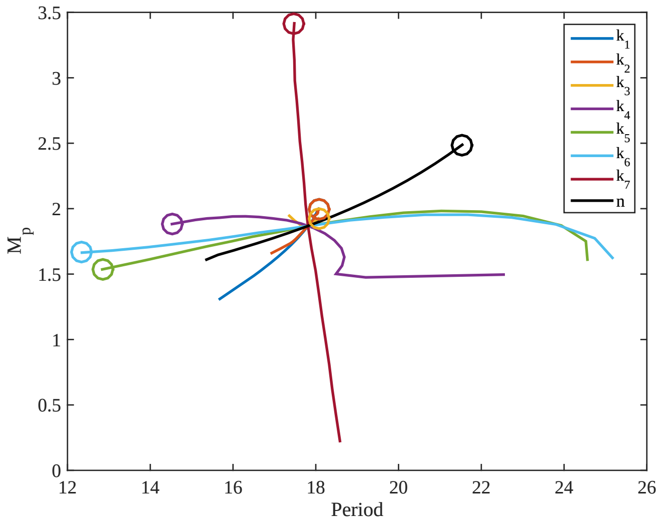


Figure 3-C : Goodwin Oscillator. Co-variation of period and amplitude metric ($M_p$). Circle shaped markers represent the largest value of the corresponding parameter. As parameter $k_1$ increases, $M_1$ and $M_p$ increases and the period slightly increases. As parameter $k_2$ increases, $M_p$ increases and the period slightly increases. As parameter $k_3$ increases, $M_p$ remains almost constant and the period does not change significantly. As parameter $k_4$ increases, $M_p$ first increases then decreases but the period decreases. As parameter $k_5$ increases, $M_p$ first increases then decreases but the period decreases. As parameter $k_6$ increases, $M_p$ first increases then decreases but the period decreases. As parameter $k_7$ increases, $M_p$ increases and the period does not change significantly. As parameter $n$ increases, $M_p$ and the period increases.

# 4 Van der Pol Oscillator

Van der Pol oscillator [4] exhibits limit-cycle oscillations and the state-space model is,

$$\begin{aligned} \dot{x}_1 &= x_2, \\ \dot{x}_2 &= \mu(1 - x_1^2)x_2 - \omega^2 x_1, \end{aligned} \tag{4}$$

with nominal values $\mu = 1$, $\omega = 1$. The maximum amplitude of $x_1$ is computed.

## 4.1 Color Maps

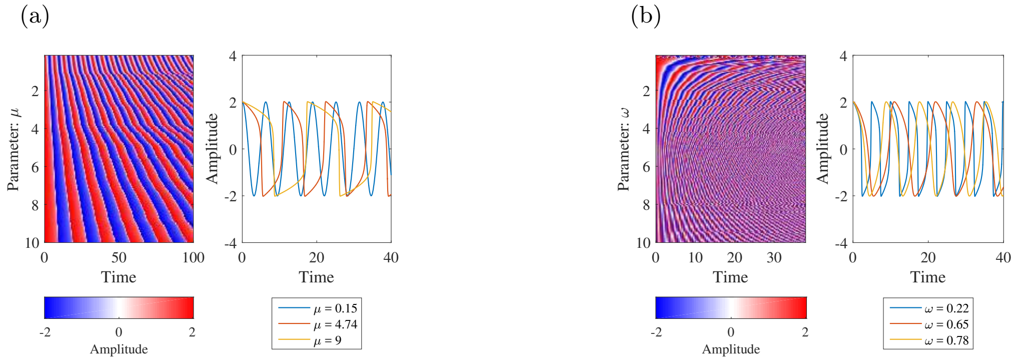


Figure 4-A : Van der Pol Oscillator. a) (left) Color-map with $\mu = 1$ to 10. (right) Trajectories for different values of $\mu$. b) (left) Color-map with $\omega = 1$ to 10. (right) Trajectories for different values of $\omega$.

## 4.2 Co-variation of period and maximum amplitude

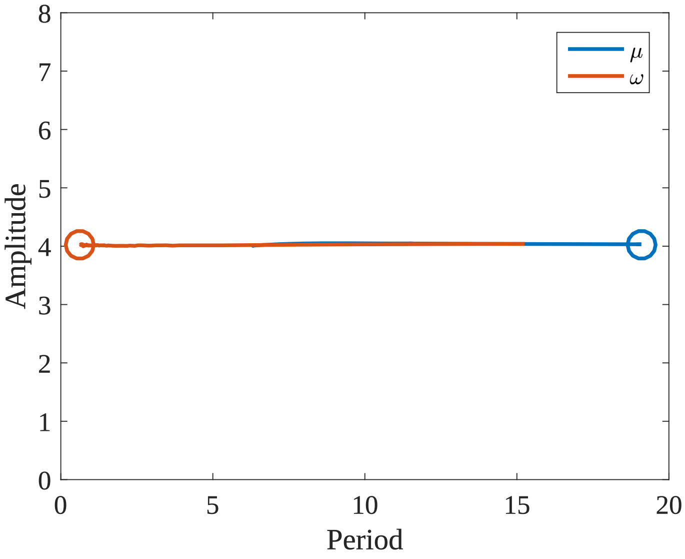


Figure 4-B : Van der Pol Oscillator. Co-variation of period and maximum amplitude. Circle shaped markers represent the largest value of the corresponding parameter. As parameter $\mu$ is increased, the amplitude remains the same but the period increases. Based on trajectories, it seems that the kind of oscillations also changes from a sinusoidal one to a square-wave one. As parameter $\omega$ is increased, the amplitude remains the same but period decreases

## 4.3 Co-variation of period and amplitude metric ($M_p$)

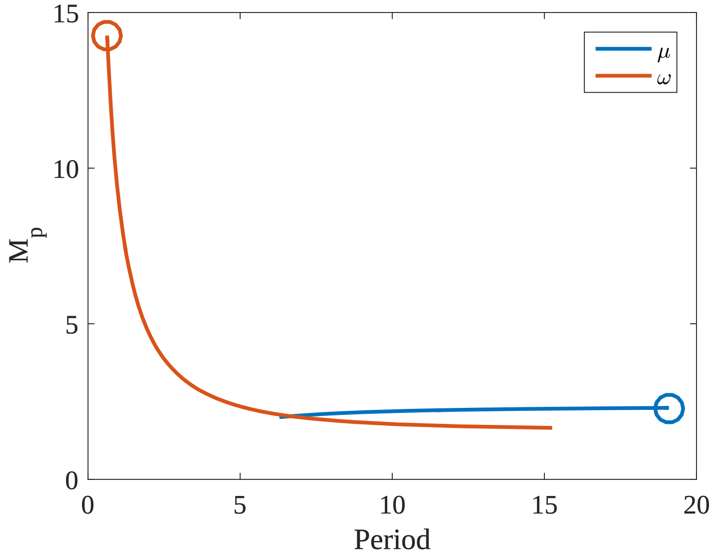


Figure 4-C : Van der Pol Oscillator. Co-variation of period and amplitude metric ($M_p$). Circle shaped markers represent the largest value of the corresponding parameter.As parameter $\mu$ is increased, $M_p$ remains constant but the period increases. As parameter $\omega$ is increased, $M_p$ increases but the period decreases.

# 5 Fitzhugh-Nagumo oscillator

Fitzhugh-Nagumo oscillator is a simplified Hodgkin-Huxley model where the dynamics of the spike neuron are given by the mathematical model [5], [6],

$$\begin{aligned} \dot{v} &= v(v-\theta)(1-v) - w + \omega, \\ \dot{w} &= \phi(v - \gamma w), \end{aligned} \tag{5}$$

with nominal values of the parameters $\theta = 0.0162$, $\omega = 0.112$, $\gamma = 2.5$, $\phi = 0.1$. Maximum amplitude of $v$ is computed.

## 5.1 Color Maps

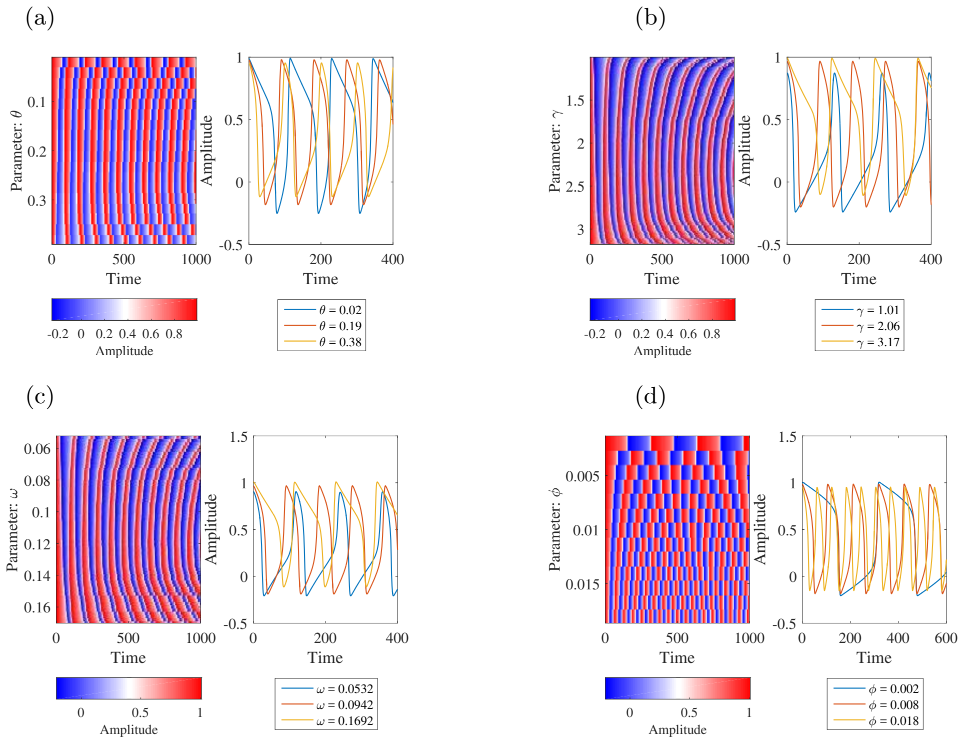


Figure 5-A : Fitzhugh-Nagumo oscillator. a) (left) Color-map with $\theta = 0.02$ to 0.38. (right) Trajectories for different values of $\theta$. b) (left) Color-map with $\gamma = 1.01$ to 3.17. (right) Trajectories for different values of $\gamma$. c) (left) Color-map with $\omega = 0.0532$ to 0.169. (right) Trajectories for different values of $\omega$. d) (left) Color-map with $\phi = 0.002$ to 0.018. (right) Trajectories for different values of $\phi$.

## 5.2 Co-variation of period and maximum amplitude

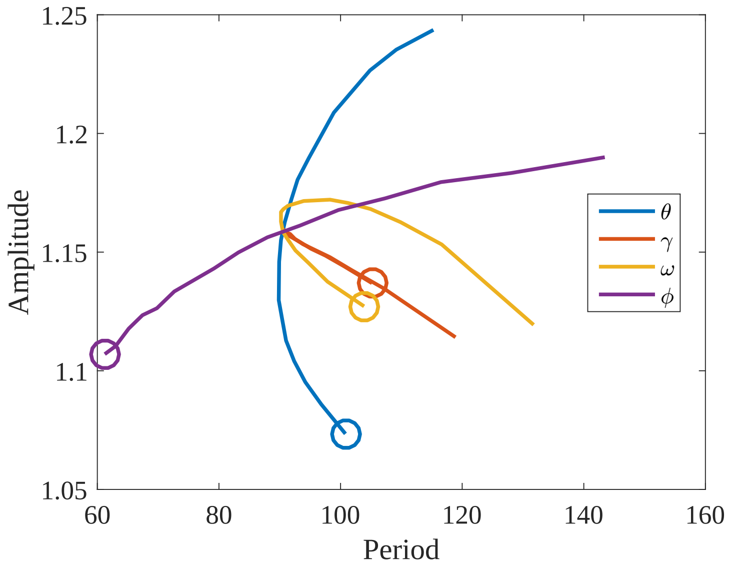


Figure 5-B : Fitzhugh-Nagumo oscillator. Co-variation of period and maximum amplitude. Circle shaped markers represent the largest value of the corresponding parameter. As parameter $\theta$ increases, the amplitude decreases and the period first decreases and then increases. As parameter $\gamma$ increases, the amplitude does not change significantly and the period first decreases then increases. As parameter $\omega$ increases, the amplitude does not change significantly and the period first decreases and then increases. As parameter $\phi$ increases, the amplitude remains the same, but the period decreases.

## 5.3 Co-variation of period and amplitude metric ($M_p$)

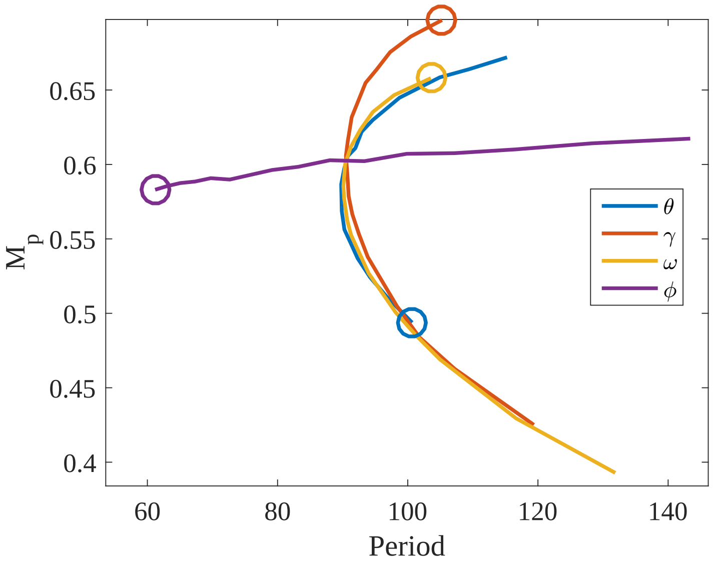


Figure 5-C : Fitzhugh-Nagumo oscillator. Co-variation of period and amplitude metric ($M_p$). Circle shaped markers represent the largest value of the corresponding parameter. As parameter $\theta$ increases, $M_p$ decreases and the period first decreases and then increases. As parameter $\gamma$ increases, $M_p$ increases and the period first decreases then increases. As parameter $\omega$ increases, $M_p$ increases and the period first decreases and then increases. As parameter $\phi$ increases, $M_p$ remains constant, but the period decreases.

# 6 Frzilator

The Frzilator is an oscillator model in which the covalent modification cascade of negative feedback to the signaling circuit of *Myxococcus xanthus* results in stable and robust oscillations for certain parameter range [7]. The mathematical model is given by Michaelis-Menten kinetic equations,

$$\begin{aligned}
\frac{df}{dt} &= \phi\left(\frac{1-f}{0.01+(1-f)}\right) - d_f\left(\frac{f}{0.005+f}\right)e, \\
\frac{dc}{dt} &= k_c\left(\frac{1-c}{0.005+(1-c)}\right)f - d_c\left(\frac{c}{0.005+c}\right), \\
\frac{de}{dt} &= k_e\left(\frac{1-e}{0.005+(1-e)}\right)c - d_e\left(\frac{e}{0.005+e}\right).
\end{aligned} \tag{6}$$

Nominal Parameters: $\phi = 0.08$. $k_c = 4$, $k_e = 4$, $d_f = 1$, $d_c = 2$ and $d_e = 2$. Maximum amplitude of $f$ is computed.

## 6.1 Color Maps

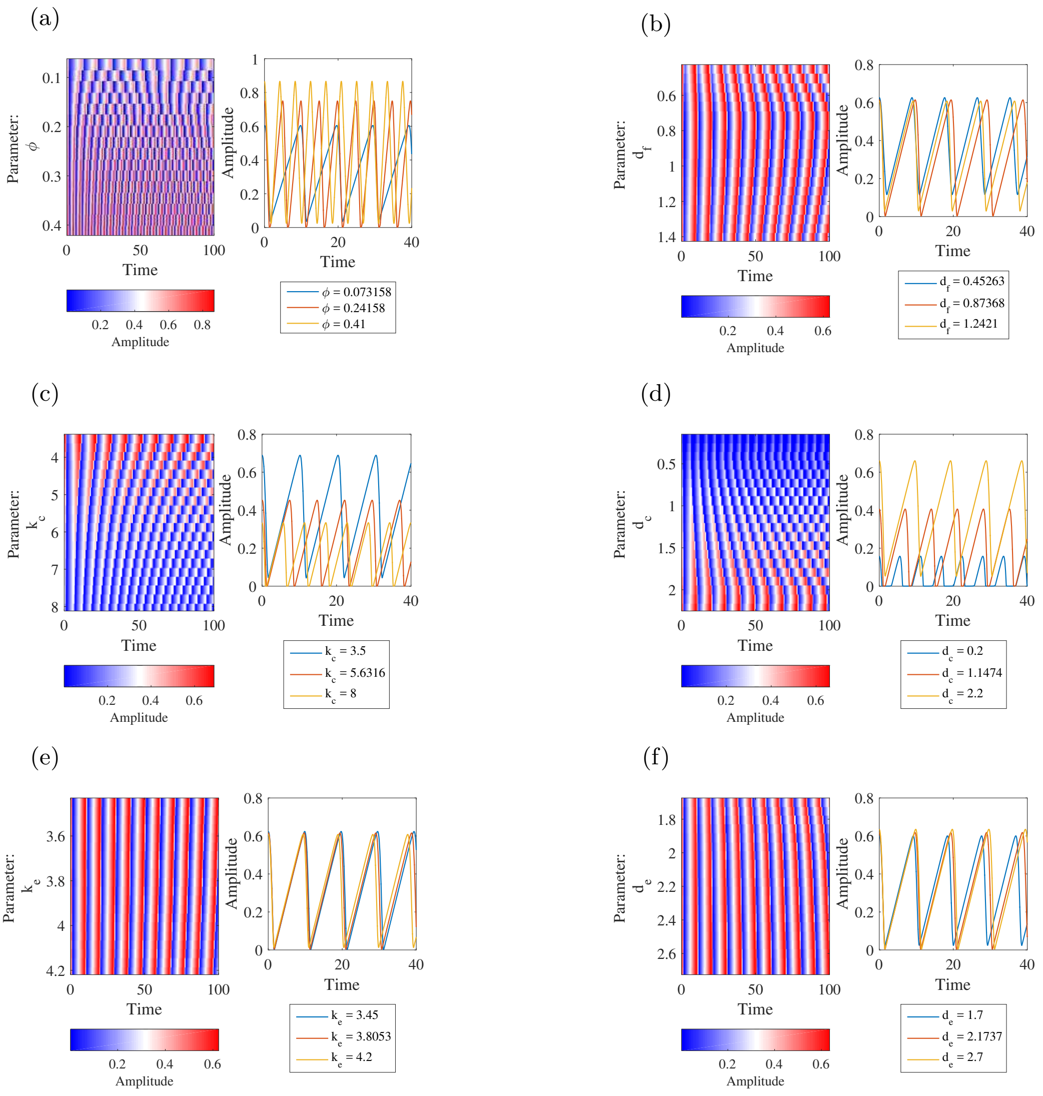


Figure 6-A : Frzilator. a) (left) Color-map with $\phi = 0.0731$ to 0.41. (right) Trajectories for different values of $\phi$. b) (left) Color-map with $d_f = 0.452$ to 1.242. (right) Trajectories for different values of $d_f$. c) (left) Color-map with $k_c = 3.5$ to 8. (right) Trajectories for different values of $k_c$. d) (left) Color-map with $d_c = 0.2$ to 2.2. (right) Trajectories for different values of $d_c$. e) (left) Color-map with $k_e = 3.45$ to 4.2. (right) Trajectories for different values of $k_e$. f) (left) Color-map with $d_e = 1.7$ to 2.7. (right) Trajectories for different values of $d_e$.

### 6.2 Co-variation of period and maximum amplitude

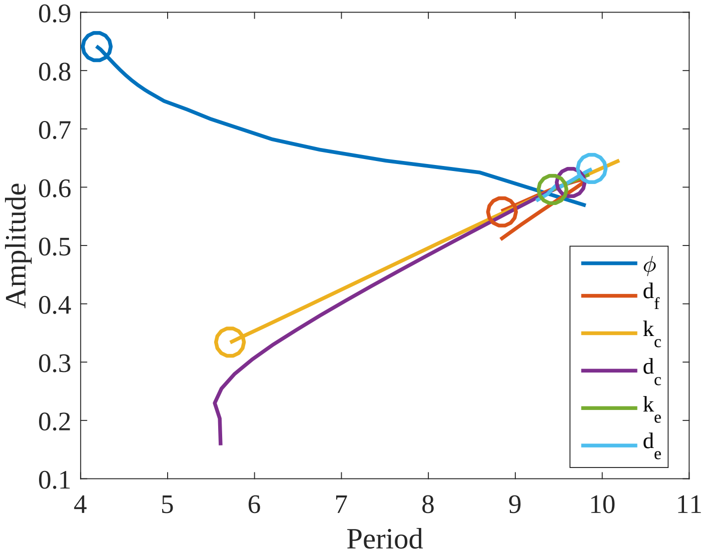


Figure 6-B : Frzilator. Co-variation of period and maximum amplitude. Circle shaped markers represent the largest value of the corresponding parameter. As parameter $\phi$ increases the amplitude increases and the period decreases. As parameter $d_f$ increases, the amplitude and period remain at similar levels. As parameter $k_c$ increases, the amplitude decreases and the period also decreases. As parameter $d_c$ increases, the amplitude increases and the period also increases. As parameter $k_e$ increases, the amplitude decreases and period also decreases. As parameter $d_e$ increases, the amplitude and period remains at similar levels.

### 6.3 Co-variation of period and amplitude metric ($M_p$)

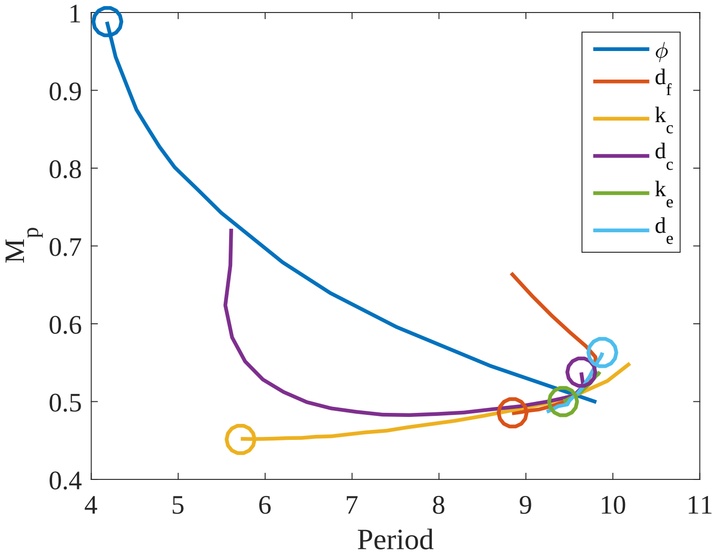


Figure 6-C : Frzilator. Co-variation of period and amplitude metric ($M_p$). Circle shaped markers represent the largest value of the corresponding parameter. As parameter $\phi$ increases, $M_p$ increases and the period decreases. As parameter $d_f$ increases, $M_p$ decreases and period first decreases then increases. As parameter $k_c$ increases, $M_p$ decreases and the period also decreases. As parameter $d_c$ increases, $M_p$ first decreases then increases and period increases. As parameter $k_e$ increases, $M_p$ and period decreases. As parameter $d_e$ increases, $M_p$ and period increases.

# 7 Cyanobacteria circadian oscillator

Circadian oscillations produced in vitro on the basis of cynobacterium *Synechococcus elongatus* using three proteins KaiA, KaiB, KaiC [8] are modeled by Rust and colleagues [9].

$$\begin{aligned}\dot{T} &= k_{UT}(S)U + k_{DT}(S)D - k_{TU}(S)T - k_{TD}(S)T,\\ \dot{D} &= k_{TD}(S)T + k_{SD}(S)S - k_{DT}(S)D - k_{DS}(S)D,\\ \dot{S} &= k_{US}(S)U + k_{DS}(S)D - k_{SU}(S)S - k_{SD}(S)S,\end{aligned} \tag{7}$$

where

$$\begin{aligned}A &= max\{0, [KaiA] - 2mS\},\\ k_{XY}(S) &= k^0_{XY} + \frac{k^A_{XY}A(S)}{K_{1/2} + A(S)}.\end{aligned} \tag{8}$$

Nominal values: $k^0_{UT} = 0.001$, $k^0_{TD} = 0.001$, $k^0_{SD} = 0.001$, $k^0_{US} = 0.001$, $k^0_{TU} = 0.21$, $k^0_{DT} = 0.001$, $k^0_{DS} = 0.31$, $k^0_{SU} = 0.11$, $k^A_{UT} = 0.479077$, $k^A_{TD} = 0.212923$, $k^A_{SD} = 0.505692$, $k^A_{US} = 0.0532308$, $k^A_{TU} = 0.0798462$, $k^A_{DT} = 0.173$, $k^A_{DS} = -0.319385$, $k^A_{SU} = -0.133077$, and $K_{1/2} = 0.43$. Maximum amplitude of $T$ is computed.

## 7.1 Color Maps

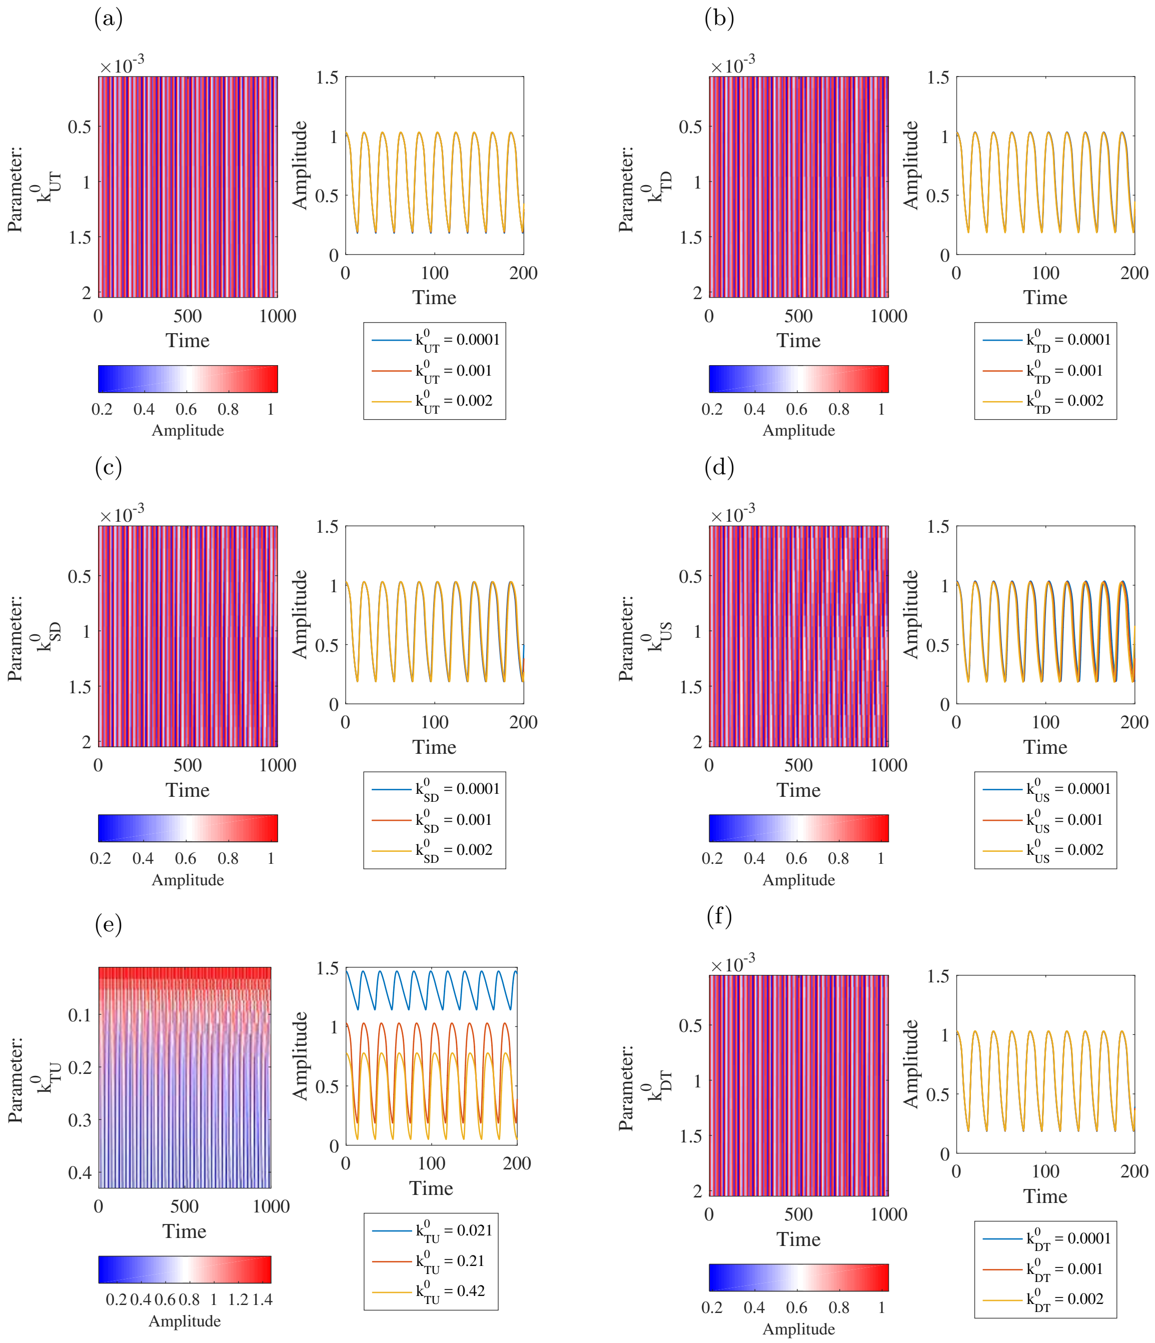


Figure 7-A : Cyanobacteria circadian oscillator. a) (left ) Color-map with $k^0_{UT} = 0.0001$ to 0.002. (right) Trajectories for different values of $k^0_{UT}$. b) (left ) Color-map with $k^0_{TD} = 0.0001$ to 0.002. (right) Trajectories for different values of $k^0_{TD}$. c) (left ) Color-map with $k^0_{SD} = 0.0001$ to 0.002. (right) Trajectories for different values of $k^0_{SD}$. d) (left ) Color-map with $k^0_{US} = 0.0001$ to 0.002. (right) Trajectories for different values of $k^0_{US}$. e) (left ) Color-map with $k^0_{TU} = 0.021$ to 0.42. (right) Trajectories for different values of $k^0_{TU}$. f) (left ) Color-map with $k^0_{DT} = 0.0001$ to 0.002. (right) Trajectories for different values of $k^0_{DT}$.

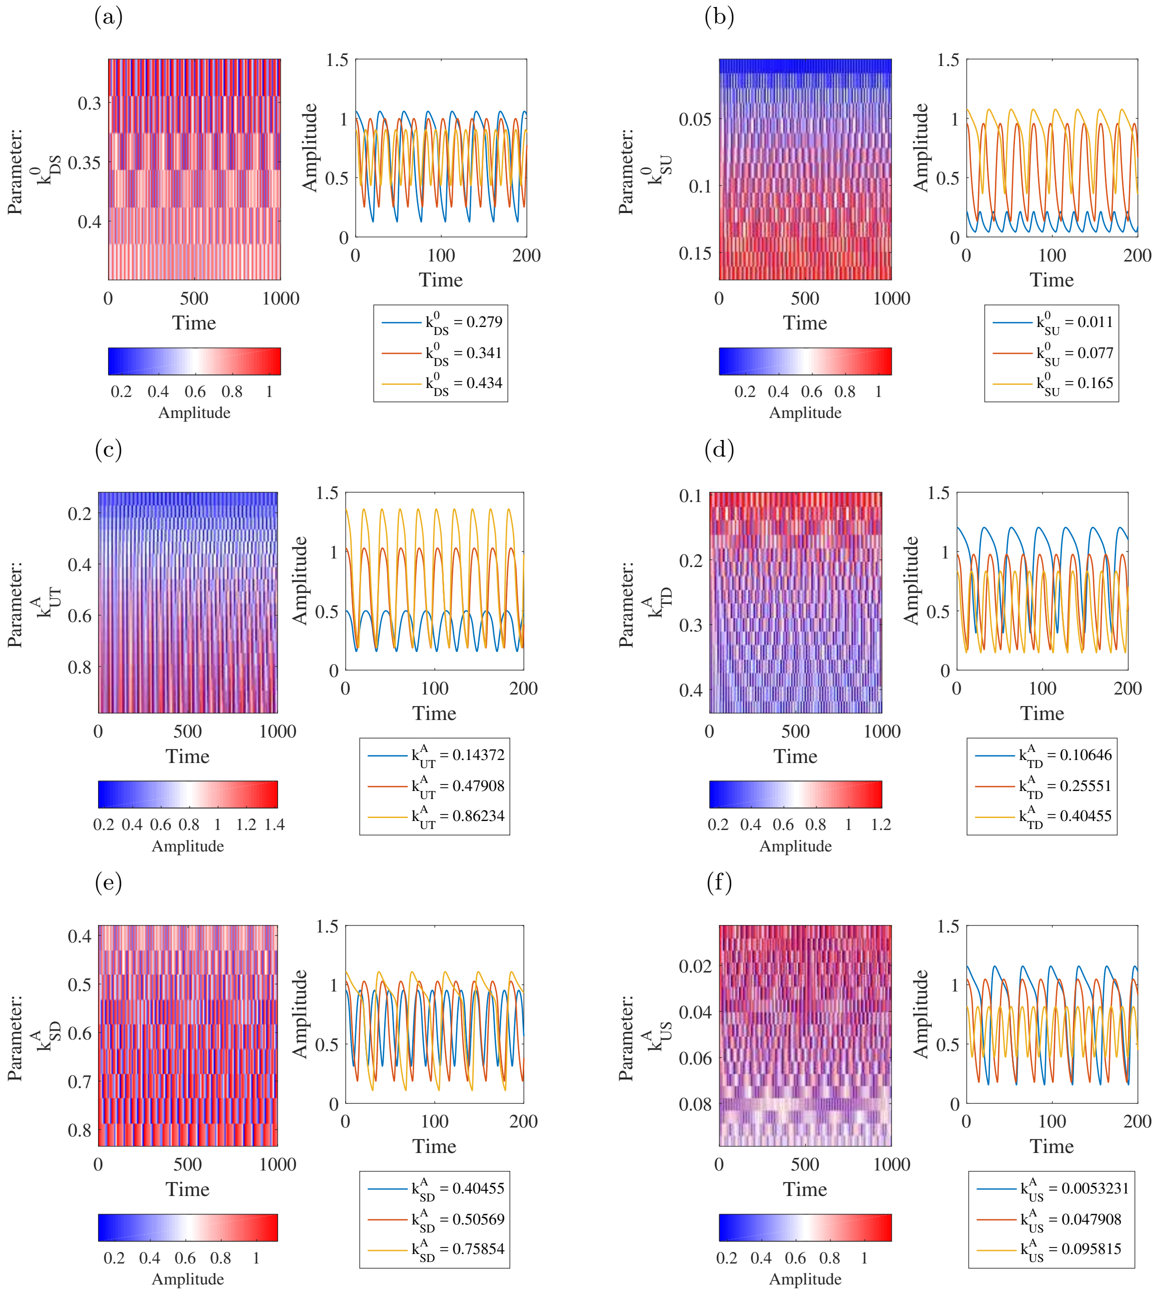


Figure 7-A (Contd.) : Cyanobacteria circadian oscillator. a) (left) Color-map with $k^0_{DS} = 0.279$ to 0.434. (right) Trajectories for different values of $k^0_{DS}$. b) (left) Color-map with $k^0_{SU} = 0.011$ to 0.165. (right) Trajectories for different values of $k^0_{SU}$. c) (left) Color-map with $k^A_{UT} = 0.14372$ to 0.8623. (right) Trajectories for different values of $k^A_{UT}$. d) (left) Color-map with $k^A_{TD} = 0.10646$ to 0.40455. (right) Trajectories for different values of $k^A_{TD}$. e) (left) Color-map with $k^A_{SD} = 0.40455$ to 0.75854. (right) Trajectories for different values of $k^A_{SD}$. f) (left) Color-map with $k^A_{US} = 0.00532$ to 0.095815. (right) Trajectories for different values of $k^A_{US}$.

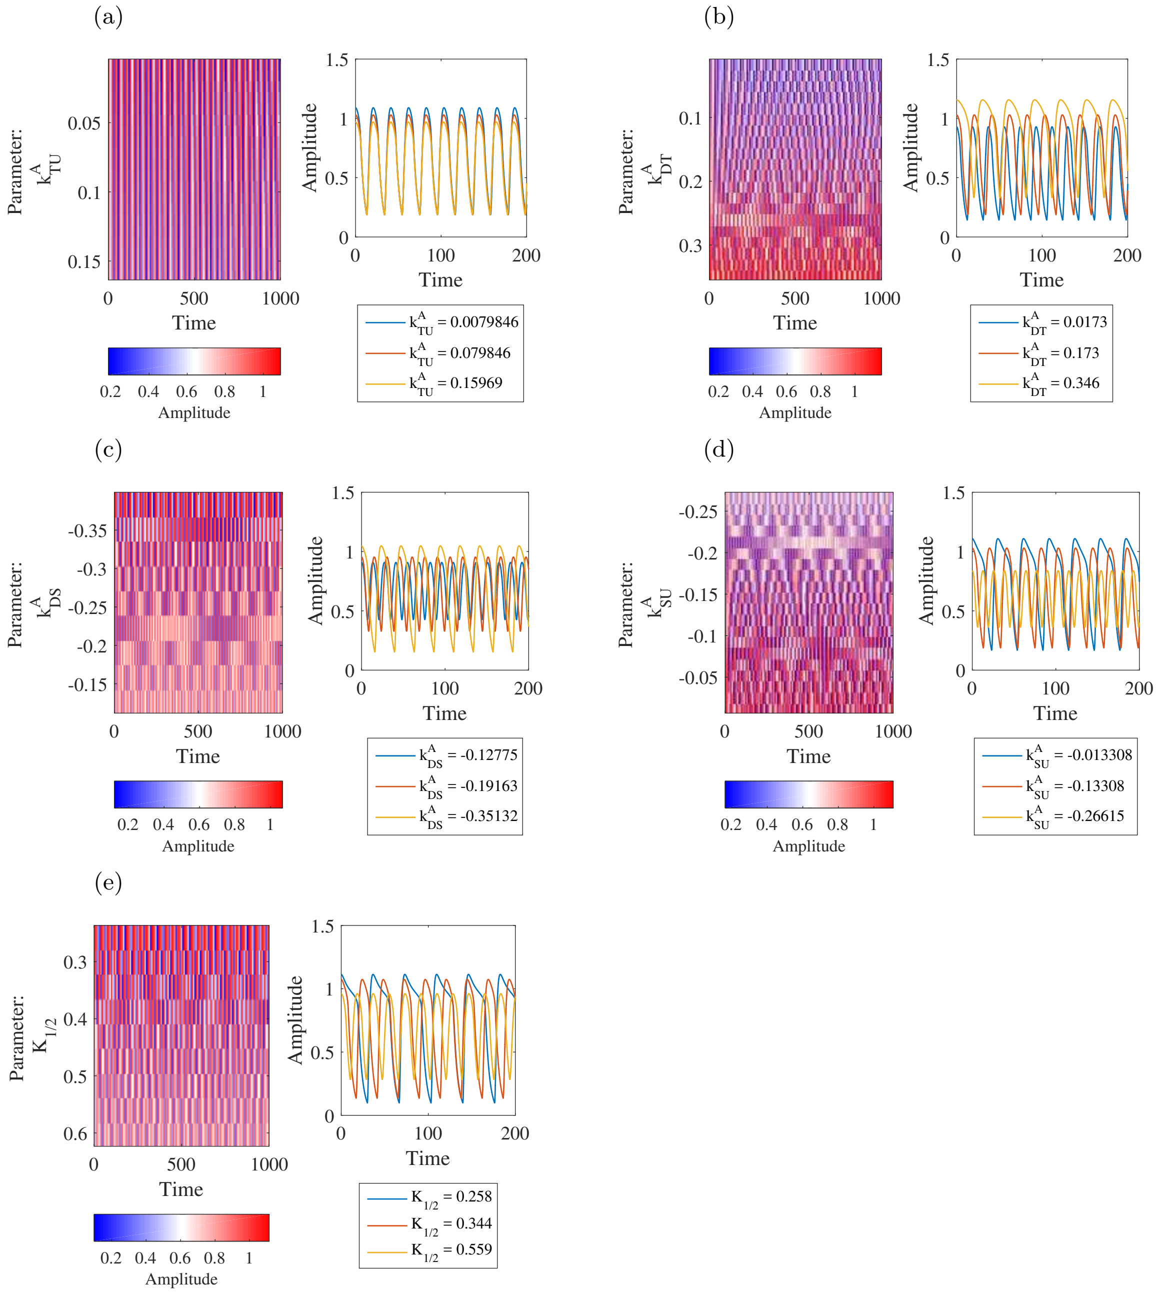


Figure 7-A (Contd.) : Cyanobacteria circadian oscillator. a) (left) Color-map with $k^A_{TU} = 0.00798$ to 0.15969. (right) Trajectories for different values of $k^A_{TU}$. b) (left) Color-map with $k^A_{DT} = 0.0173$ to 0.346. (right) Trajectories for different values of $k^A_{DT}$. c) (left) Color-map with $k^A_{DS} = -0.12775$ to $-0.35132$. (right) Trajectories for different values of $k^A_{DS}$. d) (left) Color-map with $k^A_{SU} = -0.013308$ to $-0.26615$. (right) Trajectories for different values of $k^A_{SU}$. e) (left) Color-map with $K_{1/2} = 0.258$ to 0.559. (right) Trajectories for different values of $K_{1/2}$.

## 7.2 Co-variation of period and maximum amplitude

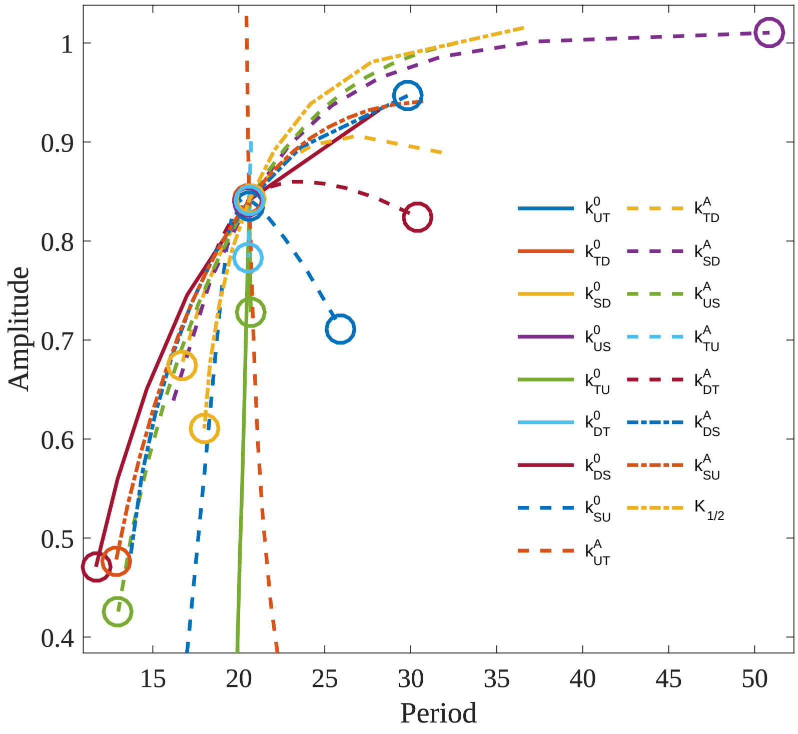


Figure 7-B : Cyanobacteria circadian oscillator. Co-variation of period and maximum amplitude. Circle shaped markers represent the largest value of the corresponding parameter. As parameters $k^0_{UT}$, $k^0_{TD}$, $k^0_{SD}$, $k^0_{US}$,$k^0_{DT}$ change, the amplitude and period do not change significantly. As $k^0_{TU}$ increases, the amplitude increases (although the average amplitude reduces), where as the period remains the same. As $k^0_{DS}$ increases, the amplitude decreases and the period also decreases. As $k^0_{SU}$ increases, the amplitude increases and the period also increases. As $k^A_{UT}$ increases, the amplitude increases and the period decreases. As $k^A_{TD}$ increases, the amplitude increases and the period decreases. As $k^A_{SD}$ increases, the amplitude increases and the period increases. As $k^A_{US}$ increases, the amplitude decreases, and the period decreases. As $k^A_{TU}$ increases, the amplitude decreases, and the period remains constant. As $k^A_{DT}$ increases, the amplitude increases and the period also increases. As $k^A_{DS}$ increases, the amplitude and period both increase. As $k^A_{SU}$ increases, the amplitude decreases and the period also decreases. As $K_{1/2}$ increases, the amplitude decreases and the period decreases.

## 7.3 Co-variation of period and amplitude metric ($M_p$)

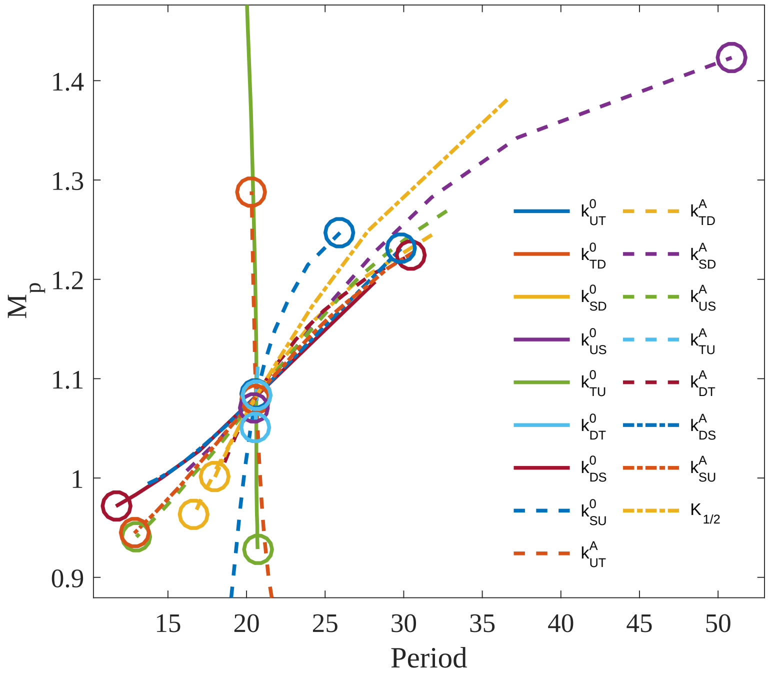


Figure 7-C : Cyanobacteria circadian oscillator. Co-variation of period and amplitude metric ($M_p$). Circle shaped markers represent the largest value of the corresponding parameter. As parameters $k^0_{UT}$, $k^0_{TD}$, $k^0_{SD}$, $k^0_{US}$,$k^0_{DT}$ change, $M_1$, $M_p$ and period do not change significantly. As $k^0_{TU}$ increases, $M_p$ decreases, where as the period remains the same. As $k^0_{DS}$ increases, $M_p$ decreases and the period also decreases. As $k^0_{SU}$ increases, $M_p$ increases and the period also increases. As $k^A_{UT}$ increases, $M_p$ increases and the period decreases. As $k^A_{TD}$ increases, $M_p$ and the period decreases. As $k^A_{SD}$ increases, $M_p$ increases and the period increases. As $k^A_{US}$ increases, $M_p$ decreases, and the period decreases. As $k^A_{TU}$ increases, $M_p$ decreases, and the period remains constant. As $k^A_{DT}$ increases, $M_p$ increases and the period also increases. As $k^A_{DS}$ increases, $M_p$ and period increase. As $k^A_{SU}$ increases, $M_p$ decreases and the period also decreases. As $K_{1/2}$ increases, $M_p$ decreases and the period decreases.

## 8 Metabolator

Metabolator [10] is a synthetic gene oscillator where the dynamics of the metabolites are expressed as,

$$\begin{aligned}
\frac{d}{dt}AcCoA &= V_{Acs} - V_{Pta} + V_{gly} - VTCA, \\
\frac{d}{dt}AcP &= V_{Pta} - VAck, \\
\frac{d}{dt}OAc^- &= V_{Ack} - V_{Ace} - VAcs, \\
\frac{d}{dt}HOAc &= V_{Ace} - Vout, \\
\frac{d}{dt}LacI &= R_{LacI} - Rd, LacI, \\
\frac{d}{dt}Pta &= R_{Pta} - Rd, Pta, \\
\frac{d}{dt}Acs &= R_{Acs} - Rd, Acs,
\end{aligned} \tag{9}$$

with

$$\begin{aligned}
V_{TCA} &= k_{TCA}AcCoA, \\
V_{Pta} &= \frac{k_1.Pta.AcCoA}{K_{m,1} + AcCoA}, \\
V_{Acs} &= \frac{k_2.Acs.OAc^-}{K_{m,2} + OAc^-}, \\
V_{Ack} &= k_{Ack,f}AcP - k_{Ack,r}OAc^-, \\
V_{Ace} &= C\left(AcPH^+ - K_{eq}OAc^-\right), \\
V_{out} &= k_3\left(HOAc - HOAc_E\right), \\
R_{LacI} &= \frac{\alpha_1\left(AcP/K_{g,1}\right)^n}{1 + \left(AcP/K_{g,1}\right)^n} + \alpha_0, \\
R_{Acs} &= \frac{\alpha_2\left(AcP/K_{g,2}\right)^n}{1 + \left(AcP/K_{g,2}\right)^n} + \alpha_0, \\
R_{Pta} &= \frac{\alpha_3}{1 + \left(LacI/K_{g,3}\right)^n} + \alpha_0, \\
R_{d,X} &= k_dX, \quad \text{with } X = LacI, Acs, Pta.
\end{aligned}$$

Nominal values of parameters: $V_{gly} = 5$, $k_{TCA} = 10$, $k_1 = 80$, $k_{m,1} = 0.06$, $k_2 = 0.8$, $k_{m,2} = 0.1$, $k_{Ack,f} = 1$, $k_{Ack,r} = 1$, $C = 100$, $H^+ = 10^{-7}$, $K_{eq} = 5 \times 10^{-4}$, $k_3 = 0.01$, $HOAC_E = 10^{-10}$, $K_{g,1} = 10$, $n = 2$, $K_{g,2} = 10$, $K_{g,3} = 0.001$, $\alpha_0 = 1e - 10$, $\alpha_1 = 0.1$, $\alpha_2 = 2$, $\alpha_3 = 2$ and $k_d = 0.06$. Maximum amplitude of $AcCoA$ is computed.

## 8.1 Color Maps

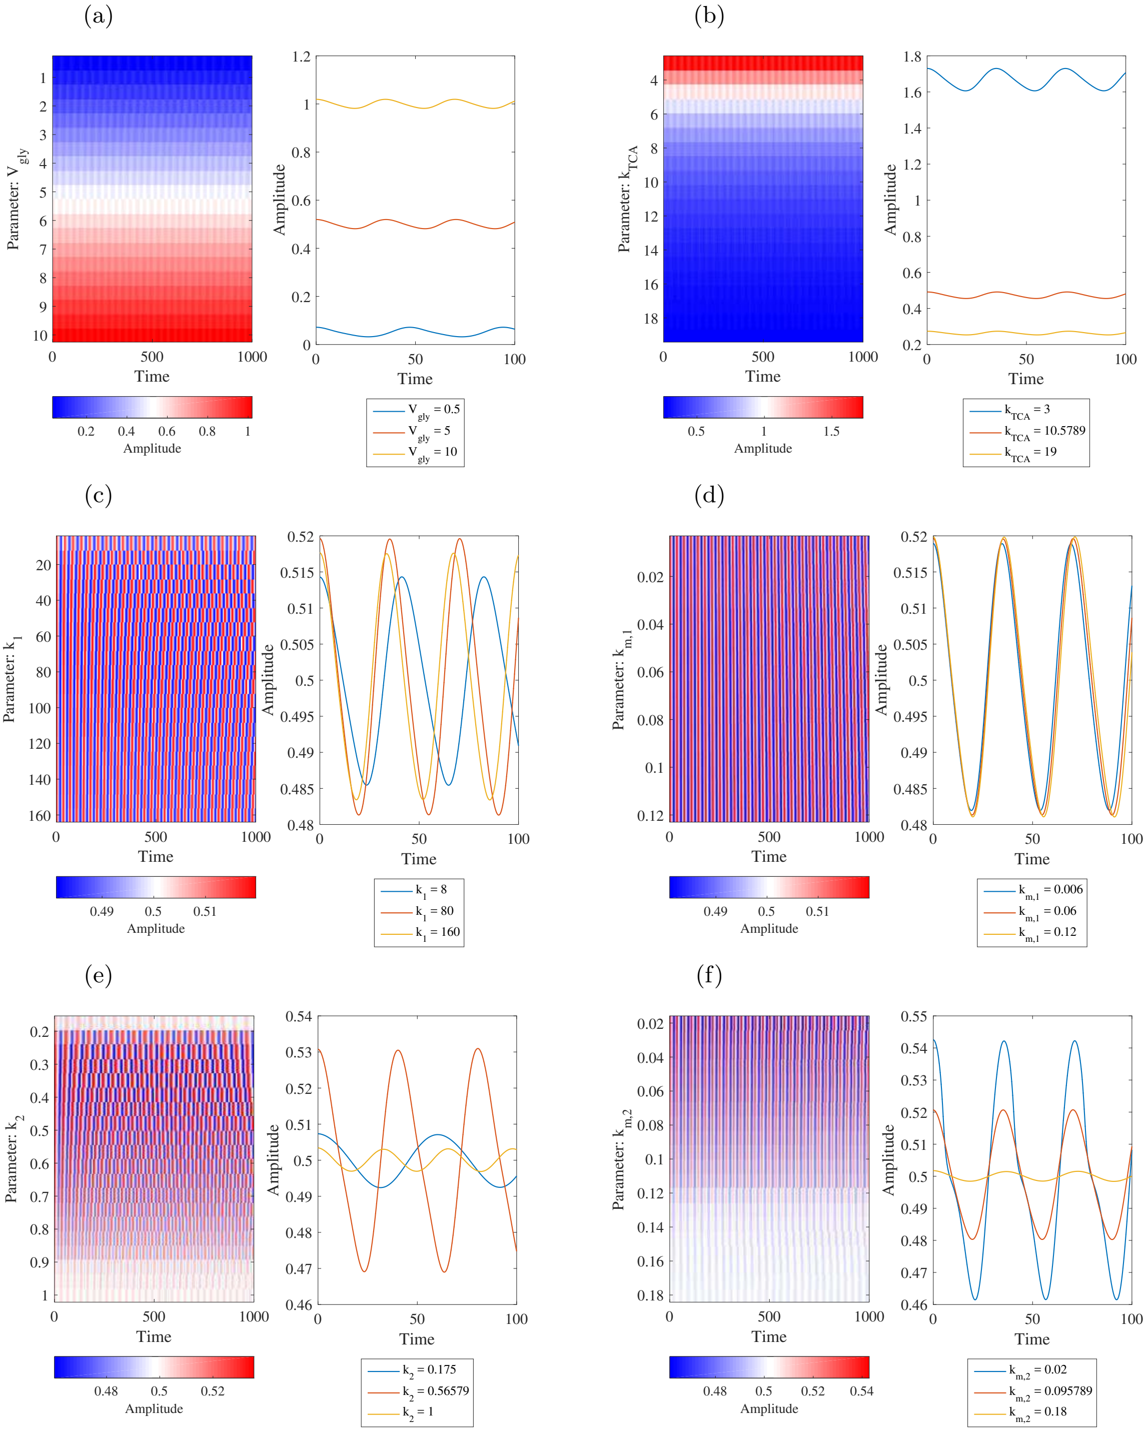


Figure 8-A : Metabolator. a) (left) Color-map with $V_{gly} = 0.5$ to 10. (right) Trajectories for different values of $V_{gly}$. b) (left ) Color-map with $k_{TCA} = 3$ to 19. (right) Trajectories for different values of $k_{TCA}$. c) (left) Color-map with $k_1 = 8$ to 160. (right) Trajectories for different values of $k_1$. d) (left) Color-map with $k_{m,1} = 0.006$ to 0.12. (right) Trajectories for different values of $k_{m,1}$. e) (left) Color-map with $k_2 = 0.175$ to 1. (right) Trajectories for different values of $k_2$. f) (left) Color-map with $k_{m,2} = 0.02$ to 0.18. (right) Trajectories for different values of $k_{m,2}$.

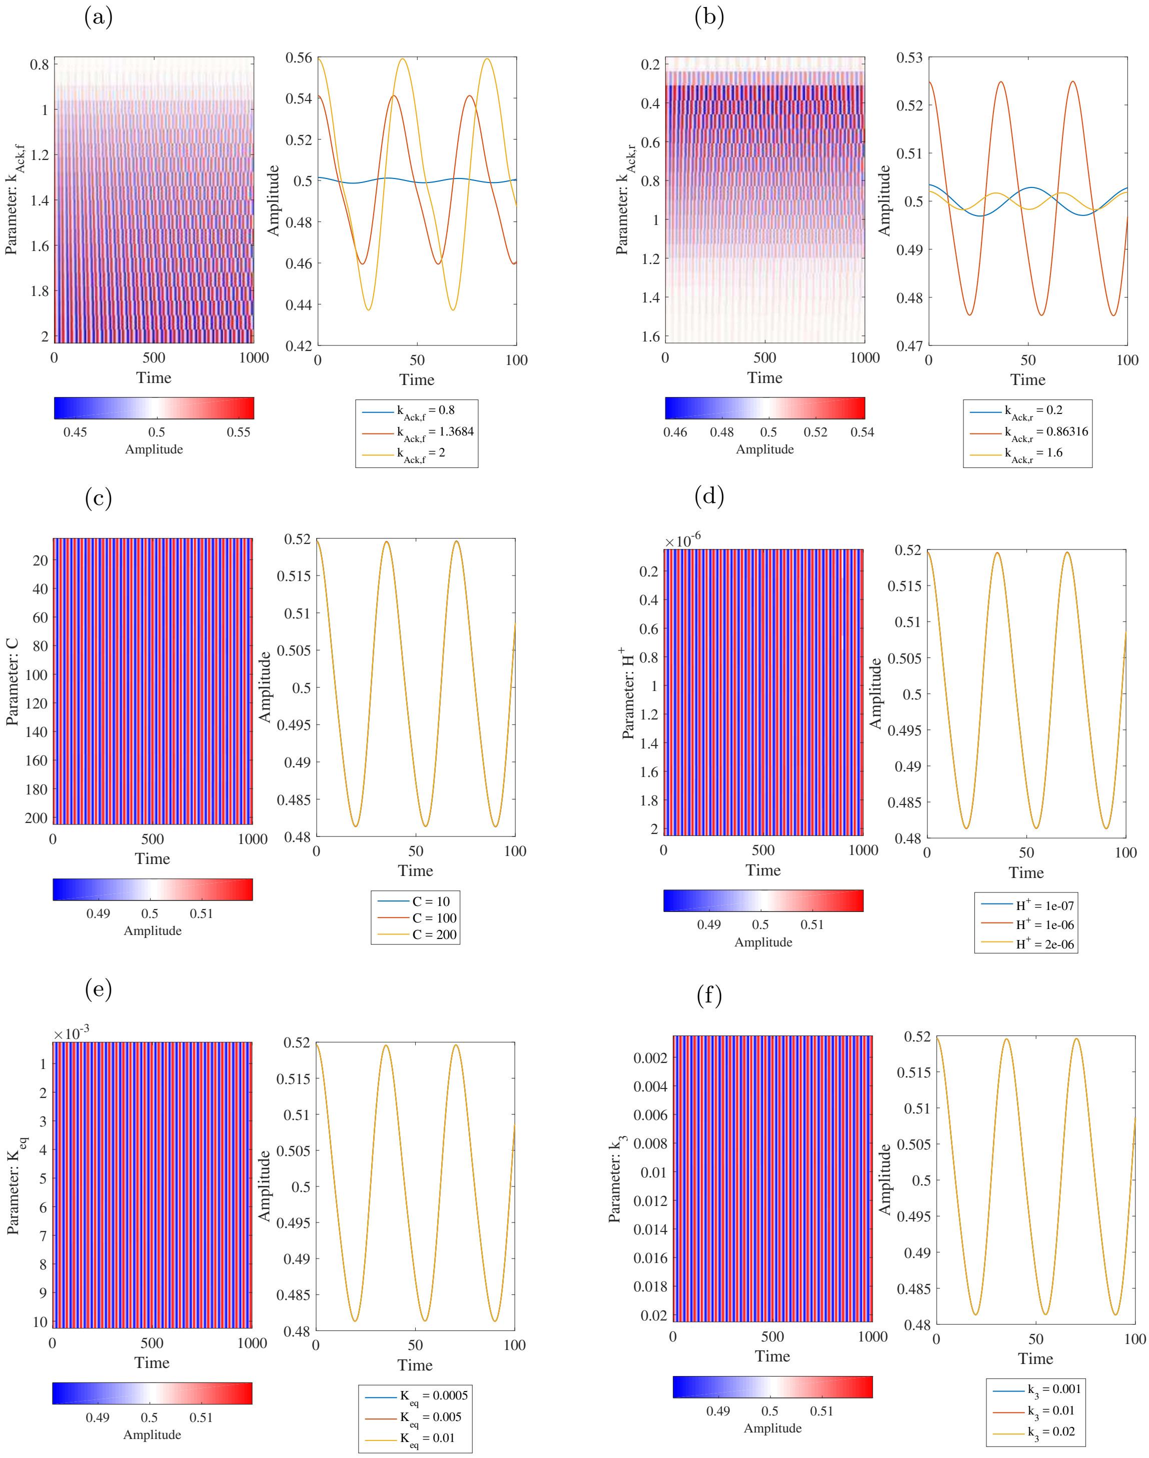


Figure 8-A (Contd.) : Metabolator. a) (left) Color-map with $k_{Ack,f} = 0.8$ to 2. (right) Trajectories for different values of $k_{Ack,f}$. b) (left) Color-map with $k_{Ack,r} = 0.2$ to 1.6. (right) Trajectories for different values of $k_{Ack,r}$. c) (left) Color-map with $C = 10$ to 100. (right) Trajectories for different values of $C$. d) (left) Color-map with $H^+ = 10^{-7}$ to $2 \times 10^{-6}$. (right) Trajectories for different values of $H^+$. e) (left) Color-map with $K_{eq} = 0.0005$ to 0.01. (right) Trajectories for different values of $K_{eq}$. f) (left) Color-map with $k_3 = 0.001$ to 0.02. (right) Trajectories for different values of $k_3$.

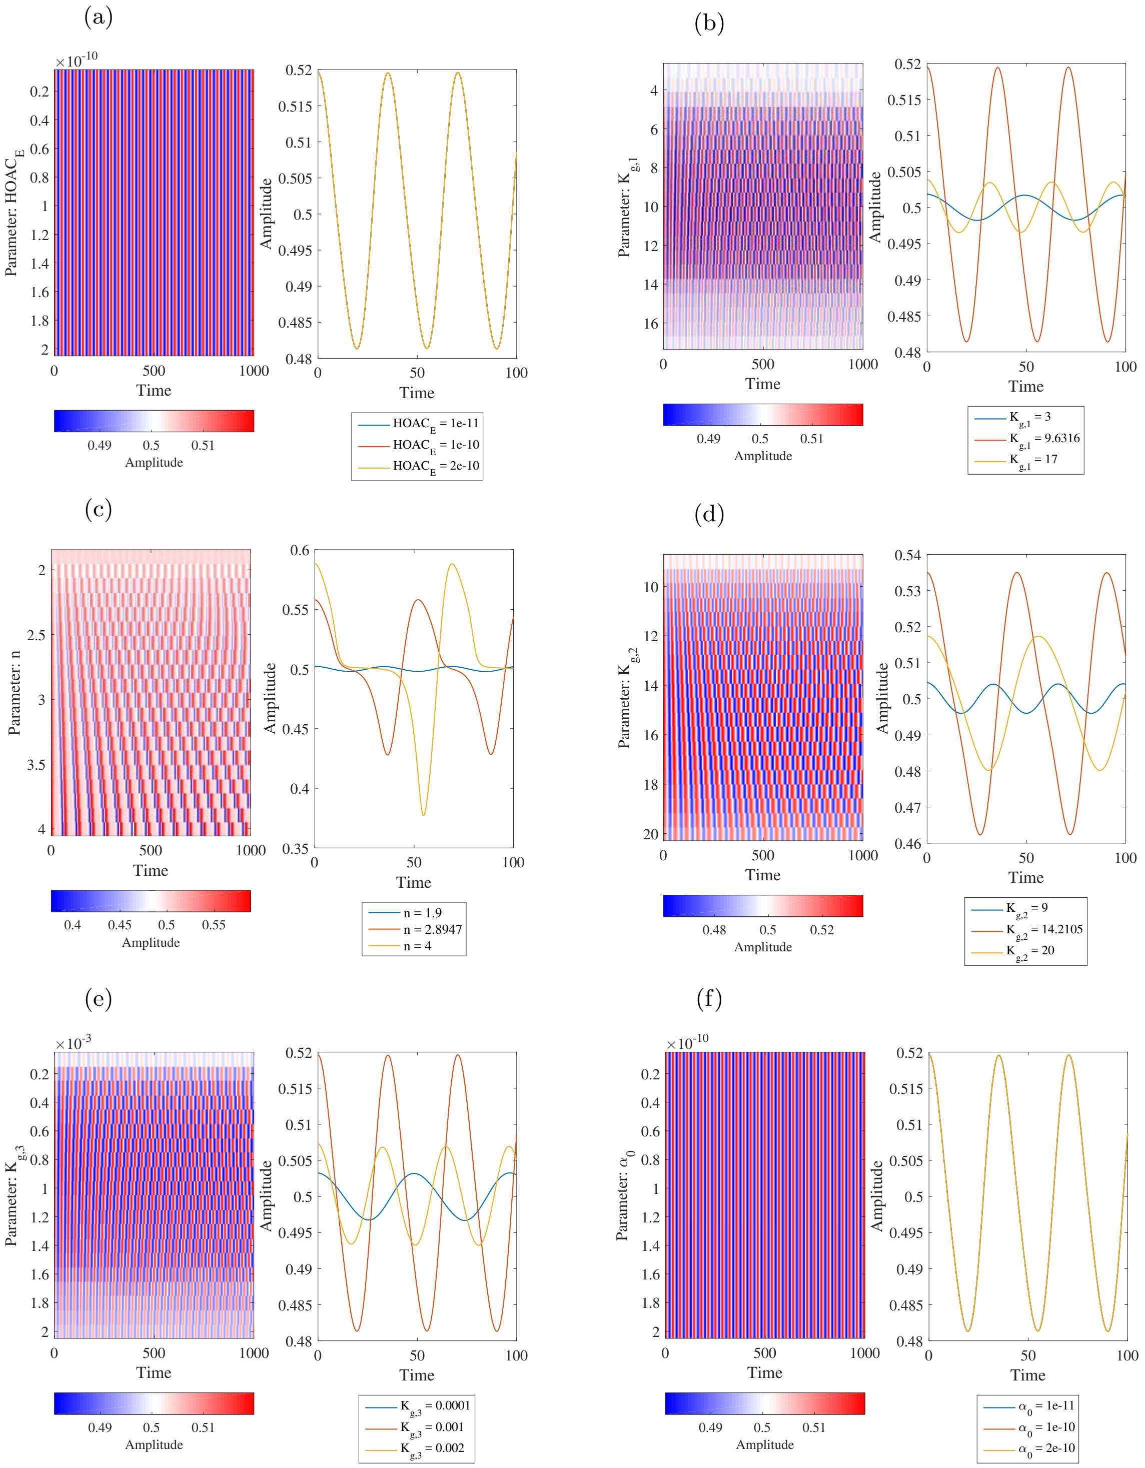


Figure 8-A (Contd.) : Metabolator. a) (left) Color-map with $HOAC_E = 10^{-11}$ to $2 \times 10^{-10}$. (right) Trajectories for different values of $HOAC_E$. b) (left) Color-map with $K_{g,1} = 3$ to 17. (right) Trajectories for different values of $K_{g,1}$. c) (left) Color-map with $n = 1.9$ to 4. (right) Trajectories for different values of $n$. d) (left) Color-map with $K_{g,2} = 9$ to 20. (right) Trajectories for different values of $K_{g,2}$. e) (left) Color-map with $K_{g,3} = 0.0001$ to 0.002. (right) Trajectories for different values of $K_{g,3}$. f) (left) Color-map with $\alpha_0 = 10^{-11}$ to $2 \times 10^{-10}$. (right) Trajectories for different values of $\alpha_0$.

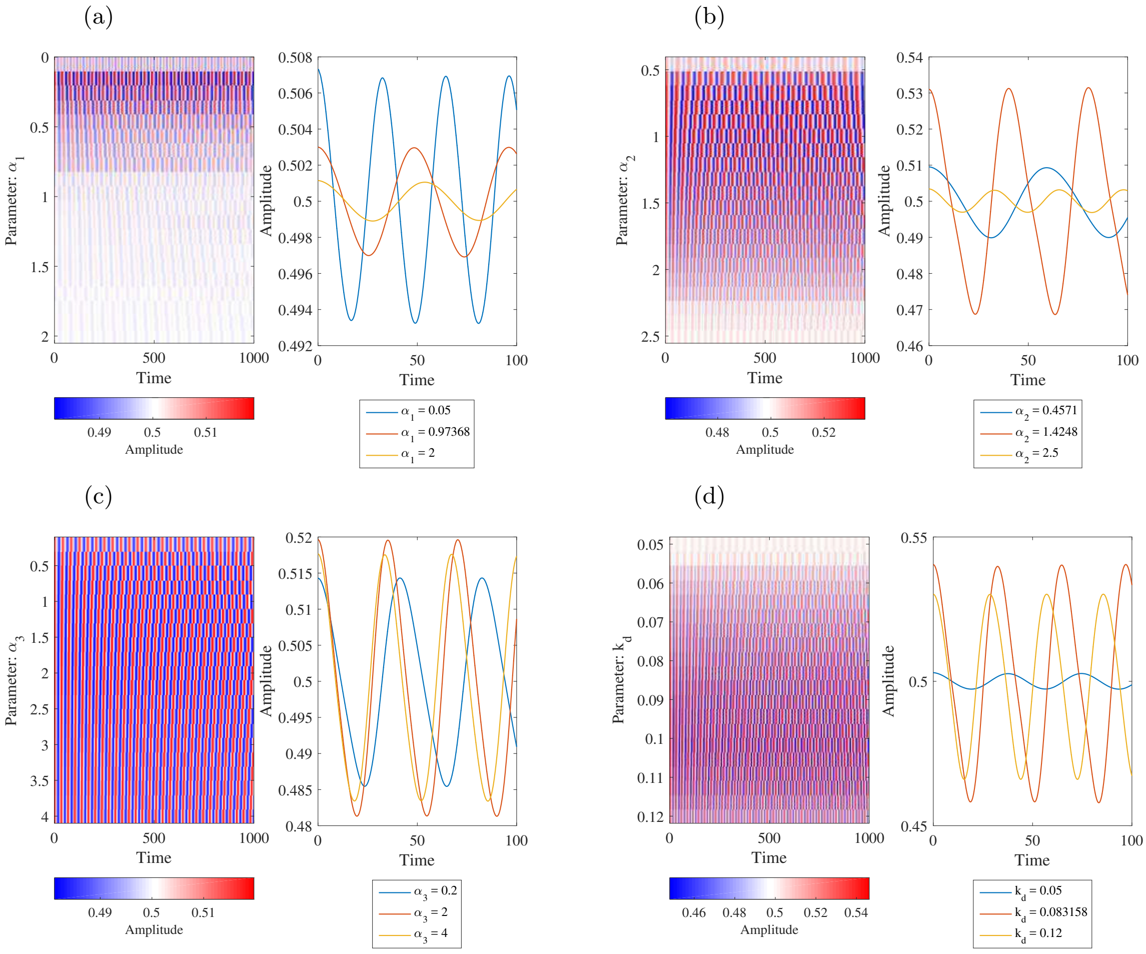


Figure 8-A (Contd.) : Metabolator. a) (left) Color-map with $\alpha_1 = 0.05$ to 2. (right) Trajectories for different values of $\alpha_1$. b) (left) Color-map with $\alpha_2 = 0.4571$ to 2.5. (right) Trajectories for different values of $\alpha_2$. c) (left) Color-map with $\alpha_3 = 0.2$ to 4. (right) Trajectories for different values of $\alpha_3$. d) (left) Color-map with $k_d = 0.05$ to 0.12. (right) Trajectories for different values of $k_d$.

## 8.2 Co-variation of period and maximum amplitude

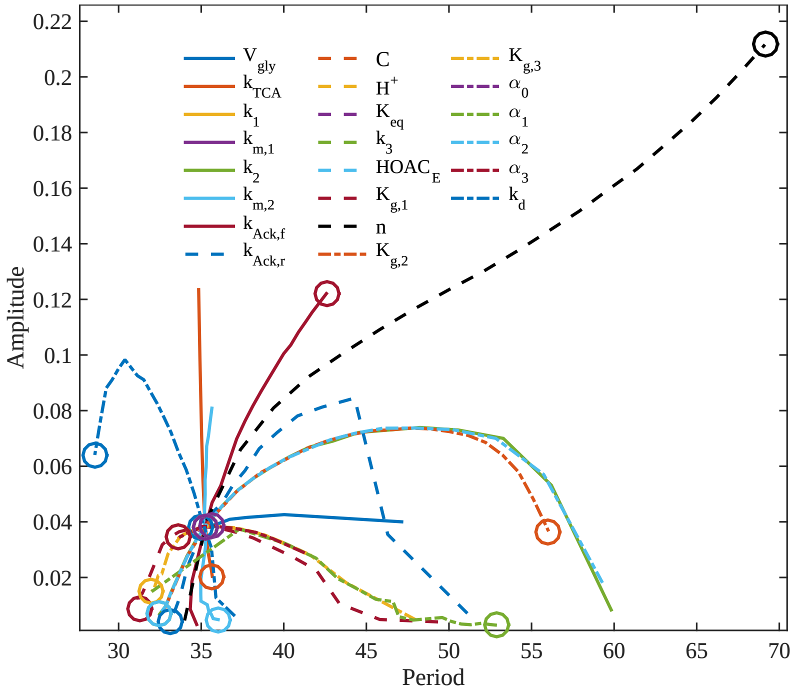


Figure 8-B : Metabolator. Co-variation of period and maximum amplitude. Circle shaped markers represent the largest value of the corresponding parameter. As parameter $V_{gly}$ increases, maximum amplitude remains similar and period decreases. As parameter $k_{TCA}$ increases, maximum amplitude decrease and the period remains at a similar level. As parameter $k_1$ increases, maximum amplitude first increases then decreases with the period decreasing. As parameter $k_{m,1}$ increases, maximum amplitude and period of the oscillator remain at similar level. As parameter $k_2$ increases, maximum amplitude first increases and then decrease with the period decreasing. As parameter $k_{m,2}$ increases, maximum amplitude decreases and the period does not change. As parameter $k_{Ack,f}$ increases, maximum amplitude increases and the period increases. As parameter $k_{Ack,r}$ increases, maximum amplitude first increases and then decreases with the period decreasing. As parameter $C$ increases, the amplitude and period remain at similar level. As parameter $H^+$ increases, the amplitude and period remain at similar level. As parameter $K_{eq}$ increases, the amplitude and period remain at similar level. As parameter $k_3$ increases, the amplitude and period remain at a similar level. As parameter $HOAC_E$ increases, the amplitude and period remain at a similar level. As parameter $K_{g,1}$ increases, the amplitude first increases then decreases, and the period decreases . As parameter $n$ increases, the amplitude increases and the period also increases. As parameter $K_{g,2}$ increases, the amplitude first increases and then decreases, and the period increases. As parameter $K_{g,3}$ increases, the amplitude first increases and then decreases, and the period decreases. As parameter $\alpha_0$ increases, the amplitude first increases and then decreases while period remains at similar value. As parameter $\alpha_1$ increases, the amplitude first increases and then decreases while period increases. As parameter $\alpha_2$ increases, the amplitude first increases then decreases, and the period decreases. As parameter $\alpha_3$ increases, the amplitude first increases and then decreases, and the period decreases. As parameter $k_d$ increases, the amplitude first increases and then decreases, and the period decreases.

## 8.3 Co-variation of period and amplitude metric ($M_p$)

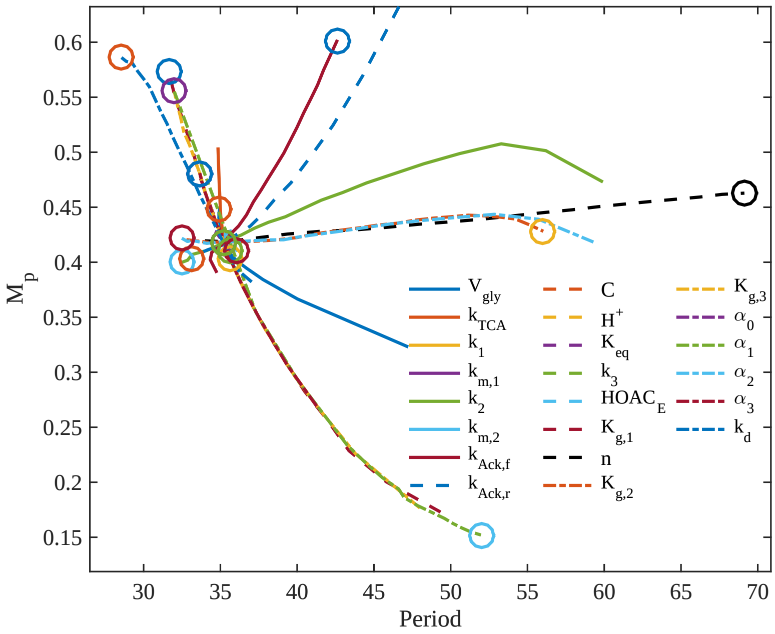


Figure 8-C Metabolator. Co-variation of period and amplitude metric ($M_p$). Circle shaped markers represent the largest value of the corresponding parameter. As parameter $V_{gly}$ increases, $M_p$ increases, while period decreases. As parameter $k_{TCA}$ increases,$M_p$ decrease and the period remains at a similar level. As parameter $k_1$ increases,$M_p$ increases with the period decreasing. As parameters $k_{m,1}$, $k_{m,2}$, $C$, $H^+$, $K_{eq}$, $k_3$, $HOAC_E$ and $\alpha_0$ increases, $M_p$ and period of the oscillator remain at similar level. As parameter $k_2$ increases,$M_p$ first increases and then decreases while the period decreases. As parameter $k_{Ack,f}$ increases, $M_p$ and the period increases. As parameter $k_{Ack,r}$ increases,$M_p$ and period decreases. As parameter $K_{g,1}$ increases, $M_p$ increases, and the period decreases. As parameter $n$ increases, $M_p$ remains constant and the period increases. As parameter $K_{g,2}$ increases, $M_p$ remains constant and the period increases. As parameter $K_{g,3}$ increases, $M_p$ increases, and the period decreases. As parameter $\alpha_1$ increases, $M_p$ decreases and period increases. As parameter $\alpha_2$ increases, $M_p$ remains constant and the period decreases. As parameter $\alpha_3$ increases, $M_p$ increases, and the period decreases. As parameter $k_d$ increases, $M_p$ increases, and the period decreases.

# 9 Mixed feedback oscillator

The synthetic gene oscillator [11] is built using gene regulatory components which gives robust oscillations. Simplified and dimensionless model is given by,

$$
\begin{aligned}
\frac{dx}{dt} &= \frac{1 + x^2 + \alpha\sigma x^4}{(1 + x^2 + \sigma x^4)(1 + y^4)} - \gamma_x x, \\
\tau_y \frac{dy}{dt} &= \frac{1 + x^2 + \alpha\sigma x^4}{(1 + x^2 + \sigma x^4)(1 + y^4)} - \gamma_y y.
\end{aligned}
\tag{10}
$$

Nominal values of parameters: $\alpha = 11$, $\sigma = 2$, $\gamma_x = 0.105$, $\gamma_y = 0.036$ and $\tau_y = 5$. Maximum amplitude of $x$ is computed.

## 9.1 Color Maps

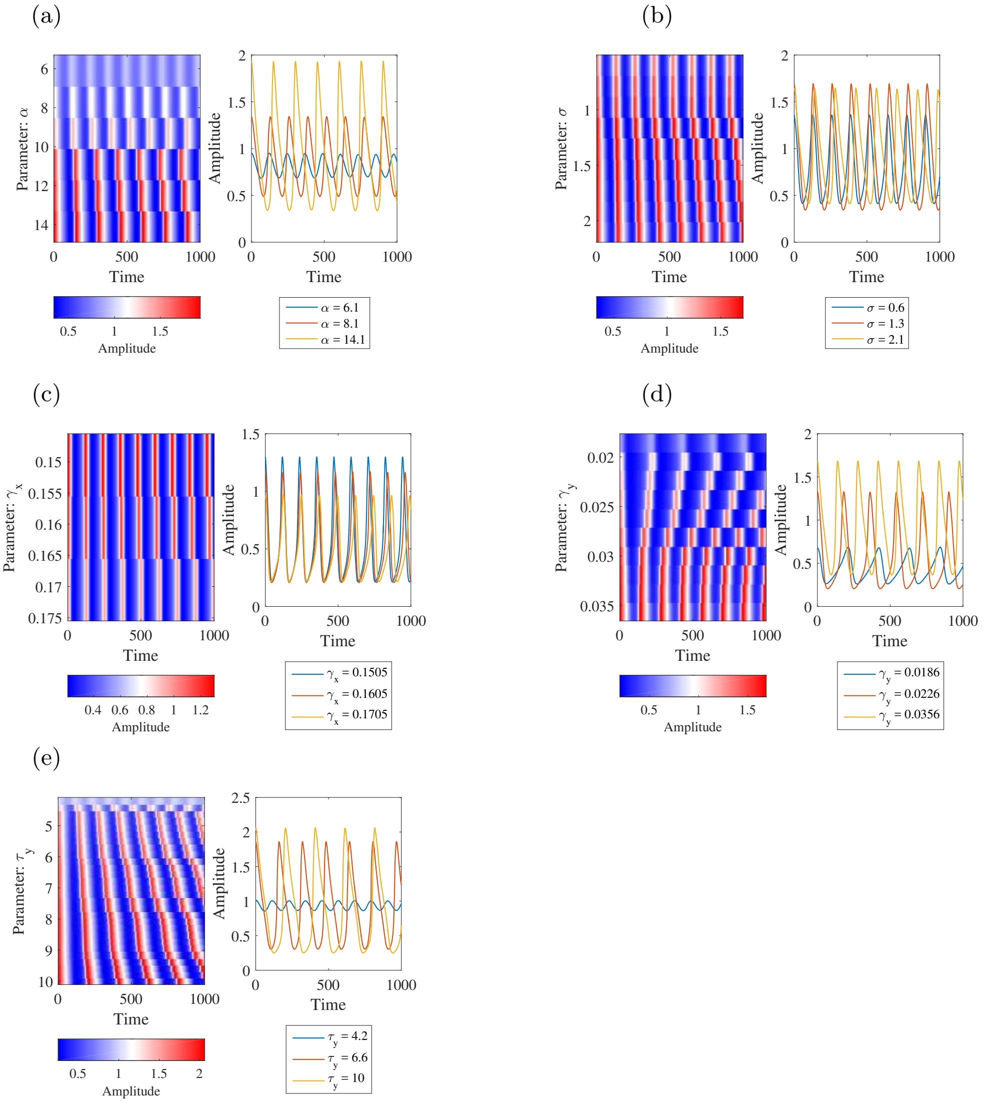


Figure 9-A : Mixed feedback oscillator. a) (left) Color-map with $\alpha = 5.79$ to 14. (right) Trajectories for different values of $\alpha$. b) (left) Color-map with $\sigma = 0.6$ to 2.12. (right) Trajectories for different values of $\sigma$. c) (left) Color-map with $\gamma_x = 0.1058$ to 0.15. (right) Trajectories for different values of $\gamma_x$. d) (left) Color-map with $\gamma_y = 0.0222$ to 0.0366. (right) Trajectories for different values of $\gamma_y$. e) (left) Color-map with $\tau_y = 4.2$ to 10. (right) Trajectories for different values of $\tau_y$.

## 9.2 Co-variation of period and maximum amplitude

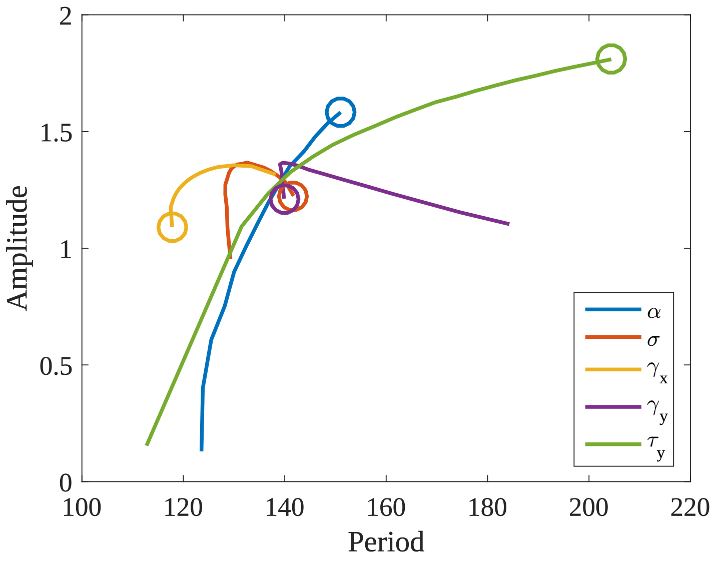


Figure 9-B : Mixed feedback oscillator. Co-variation of period and maximum amplitude. Circle shaped markers represent the largest value of the corresponding parameter. As parameter $\alpha$ increases, the amplitude increases and the period increases. As parameter $\sigma$ increases, the amplitude first increases and then decreases while the period remains constant. As parameter $\gamma_x$ increases, the amplitude decreases and the period decreases. As parameter $\gamma_y$ increases, the amplitude increases and the period decreases. As parameter $\tau_y$ increases, the amplitude increases and the period increases.

## 9.3 Co-variation of period and amplitude metric ($M_p$)

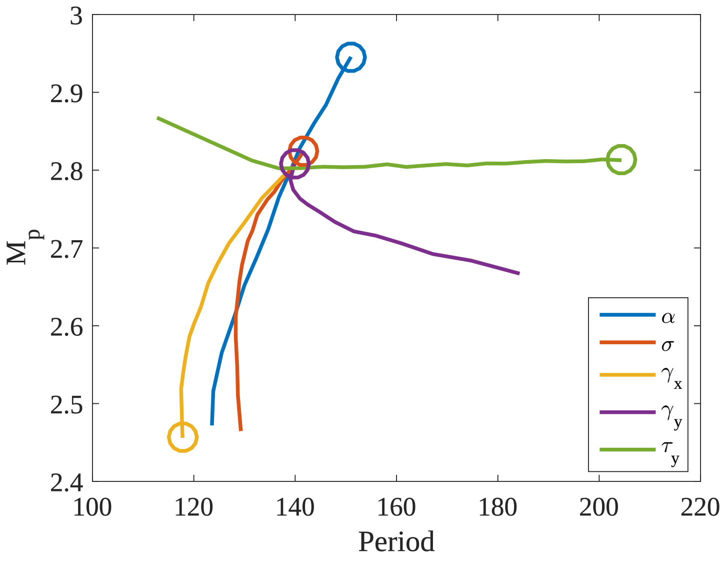


Figure 9-C : Mixed feedback oscillator. Co-variation of period and amplitude metric ($M_p$). Circle shaped markers represent the largest value of the corresponding parameter. As parameter $\alpha$ increases, $M_p$ increases and the period increases. As parameter $\sigma$ increases, $M_p$ increases and period increases. As parameter $\gamma_x$ increases, $M_p$ decreases and the period decreases. As parameter $\gamma_y$ increases, $M_p$ increases and the period decreases. As parameter $\tau_y$ increases, $M_p$ remains constant and the period increases.

# 10 Meyer and Stryer model of calcium oscillations

In this model, oscillations in calcium concentration levels [12] are observed and the dynamics are described by,

$$\begin{aligned}
\frac{dx}{dt} &= c_1 \frac{y^3}{(K_1+y)^3} z - c_2 \frac{x^2}{(K_2+x)^2} + c_3 z^2 - c_6 (\frac{x}{c_7})^{3.3} + c_6, \\
\frac{dy}{dt} &= c_4 R \frac{x}{(K_3+x)} - c_5 y, \\
\frac{dz}{dt} &= -c_1 \frac{y^3}{(K_1+y)^3} z + c_2 \frac{x^2}{(K_2+x)^2} - c_3 z^2.
\end{aligned} \tag{11}$$

Nominal Parameters: $c_1 = 6.64$, $c_2 = 5$, $c_3 = 0.0000313$, $c_4 = 1$, $c_5 = 2$, $c_6 = 0.5$, $c_7 = 0.6$, $K_1 = 0.1$, $K_2 = 0.15$, $K_3 = 1$ and $R = 0.25$. Maximum amplitude of $x$ is computed.

## 10.1 Color Maps

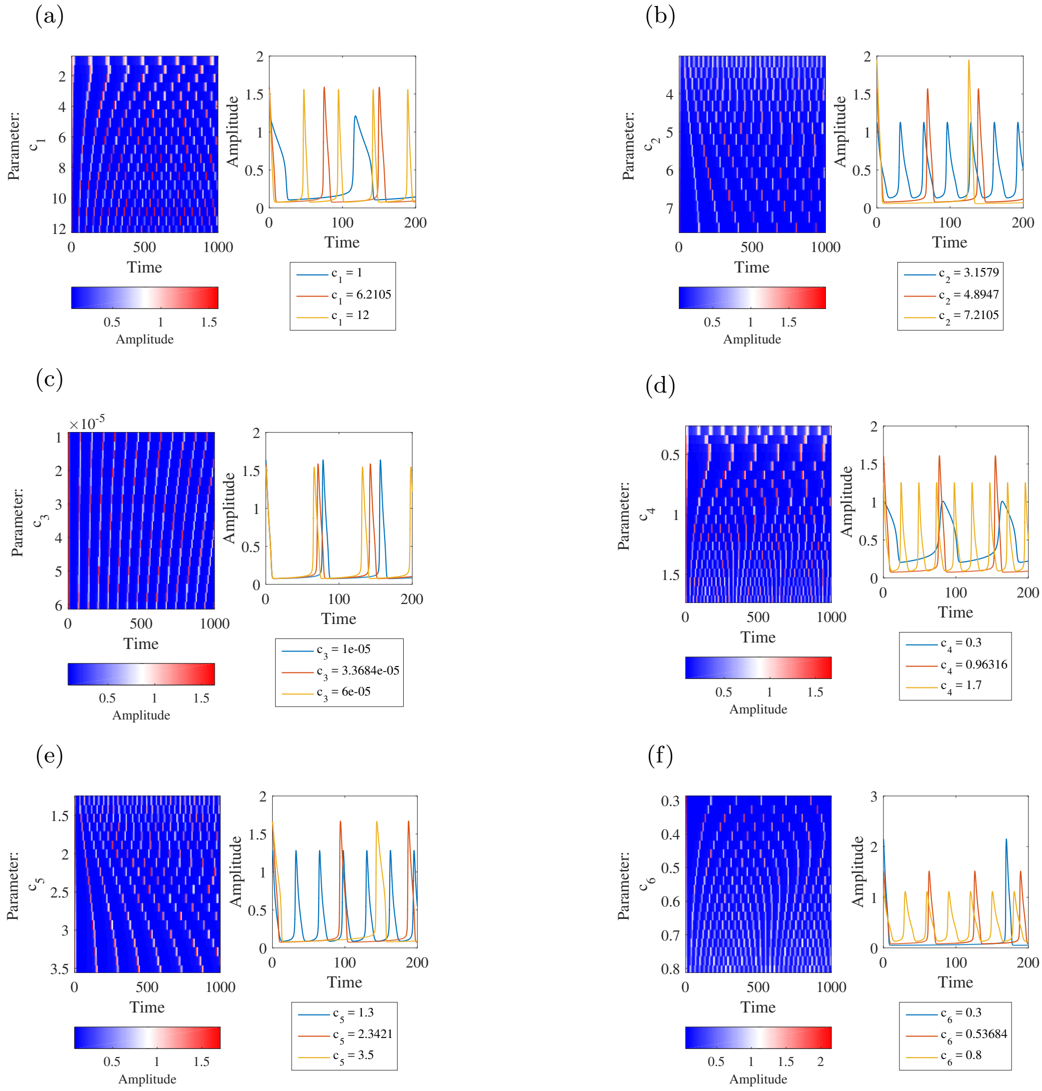


Figure 10-A : Meyer and Stryer model. a) (left) Color-map with $c_1 = 1$ to 12. (right) Trajectories for different values of $c_1$. b) (left) Color-map with $c_2 = 3.15$ to 7.21. (right) Trajectories for different values of $c_2$. c) (left) Color-map with $c_3 = 10^{-5}$ to $6 \times 10^{-5}$. (right) Trajectories for different values of $c_3$. d) (left) Color-map with $c_4 = 0.3$ to 1.7. (right) Trajectories for different values of $c_4$. e) (left) Color-map with $c_5 = 1.3$ to 3.5. (right) Trajectories for different values of $c_5$. f) (left) Color-map with $c_6 = 0.3$ to 0.8. (right) Trajectories for different values of $c_6$.

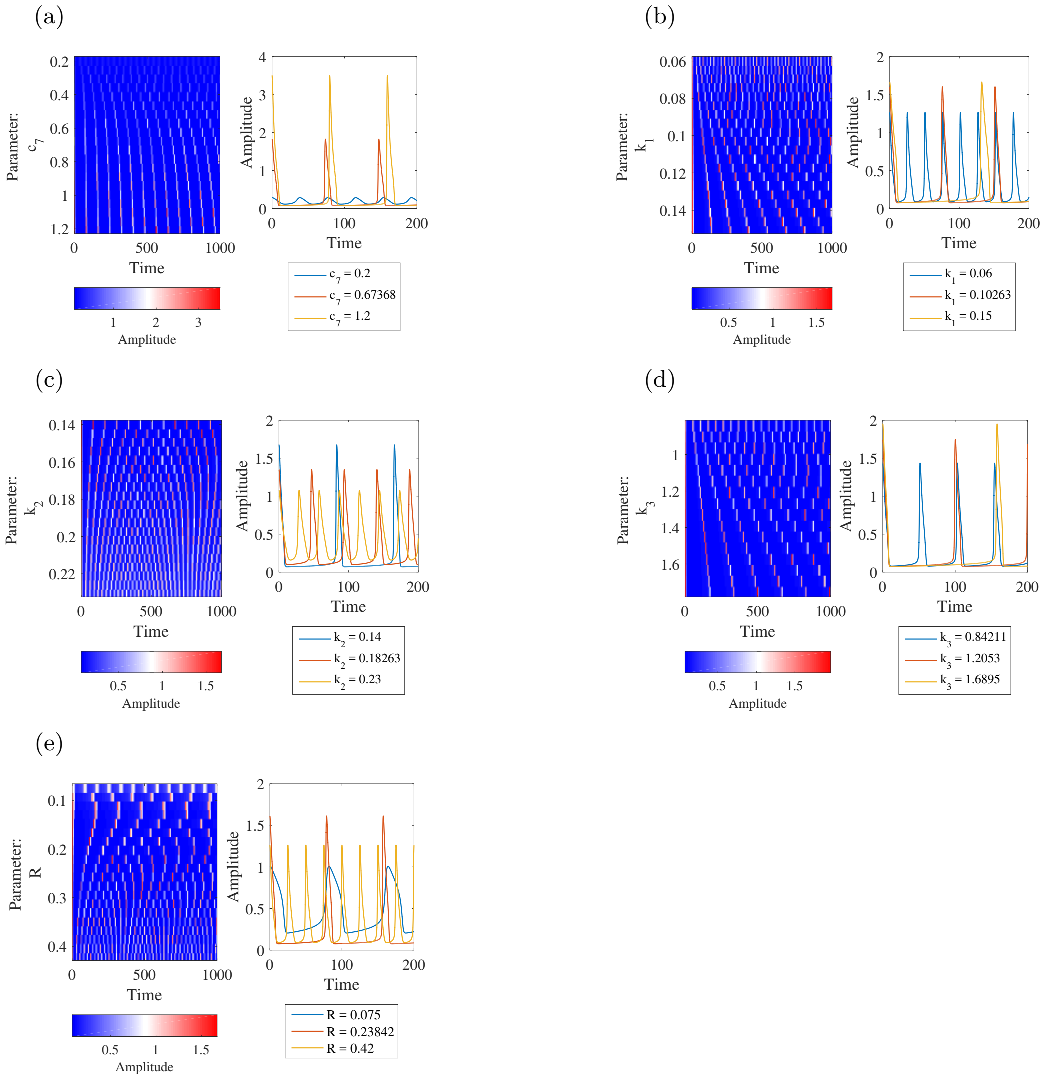


Figure 10-A (Contd.) : Meyer and Stryer model. a) (left) Color-map with $c_7 = 0.2$ to 1.2. (right) Trajectories for different values of $c_7$.b) (left) Color-map with $k_1 = 0.06$ to 0.15. (right) Trajectories for different values of $k_1$. c) (left) Color-map with $k_2 = 0.14$ to 0.23. (right) Trajectories for different values of $k_2$.d) (left) Color-map with $k_3 = 0.84$ to 1.69. (right) Trajectories for different values of $k_3$. e) (left) Color-map with $R = 0.075$ to 0.42. (right) Trajectories for different values of $R$.

## 10.2 Co-variation of period and maximum amplitude

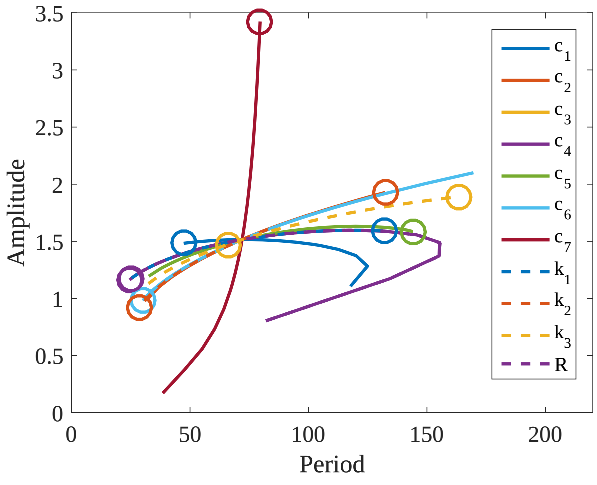


Figure 10-B : Meyer and Stryer model. Co-variation of period and maximum amplitude. Circle shaped markers represent the largest value of the corresponding parameter. As parameter $c_1$ increases, the amplitude increases and the period decreases. As parameter $c_2$ increases, the amplitude increases and the period increases. As parameter $c_3$ increases, the both the amplitude remains constant while period decreases. As parameter $c_4$ increases, the amplitude and period both first increase and then decrease. As parameter $c_5$ increases, the amplitude and period both increase. As parameter $c_6$ increases, the amplitude decreases and the period also decreases. As parameter $c_7$ increases, the amplitude and period both increase. As parameter $K_1$ increases, the amplitude and period both increase. As parameter $K_2$ increases, the amplitude and period both decrease. As parameter $K_3$ increases, the amplitude and the period both increase. As parameter $R$ increases, the amplitude and period both first increase then decrease.

## 10.3 Co-variation of period and amplitude metric ($M_p$)

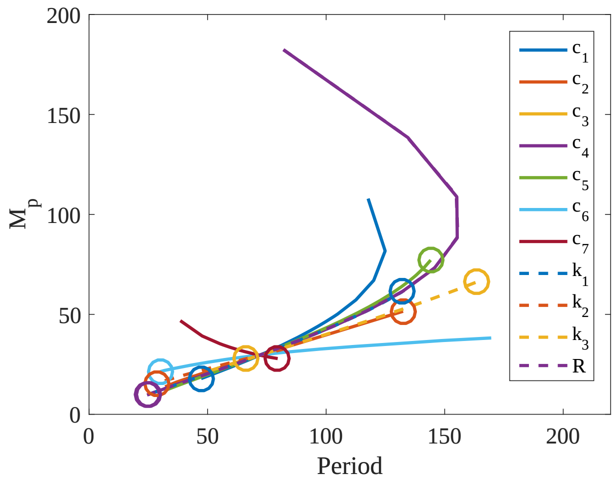


Figure 10-C : Meyer and Stryer model. Co-variation of period and amplitude metric ($M_p$). Circle shaped markers represent the largest value of the corresponding parameter. As parameter $c_1$ increases, $M_p$ decreases and the period decreases. As parameter $c_2$ increases, $M_p$ increases and the period increases. As parameter $c_3$ increases, $M_p$ and period decreases to a small extent. As parameter $c_4$ increases, $M_p$ decreases and period first increases then decreases. As parameter $c_5$ increases, $M_p$ and period increase. As parameter $c_6$ increases, $M_p$ decreases and the period also decreases. As parameter $c_7$ increases, $M_p$ decreases and period increases. As parameter $K_1$ increases, $M_p$ and period increase. As parameter $K_2$ increases, $M_p$ and period decrease. As parameter $K_3$ increases, $M_p$ and period increase. As parameter $R$ increases, $M_p$ decreases and period first increases then decreases.

## 11 Kim-Forger model

Kim-Forger model describes a protein-sequestration based repression mechanism that can be used to model circadian type oscillations [13].

$$\begin{aligned}
\dot{x} &= k_1 f(z) - k_4 x \\
\dot{y} &= k_2 x - k_5 y \\
\dot{z} &= k_3 y - k_6 z \\
f(z) &= \frac{k_7 - k_8 - z + \sqrt{(k_7 - k_8 - z)^2 + 4k_7k_8}}{2k_7}
\end{aligned} \tag{12}$$

with $k_1 = k_2 = k_3 = 1$, $k_4 = 0.16$, $k_5 = 0.29$, $k_6 = 0.3$, $k_7 = 0.6$ and $k_8 = 10^{-5}$. Maximum amplitude of protein $y$ is computed.

## 11.1 Color Maps

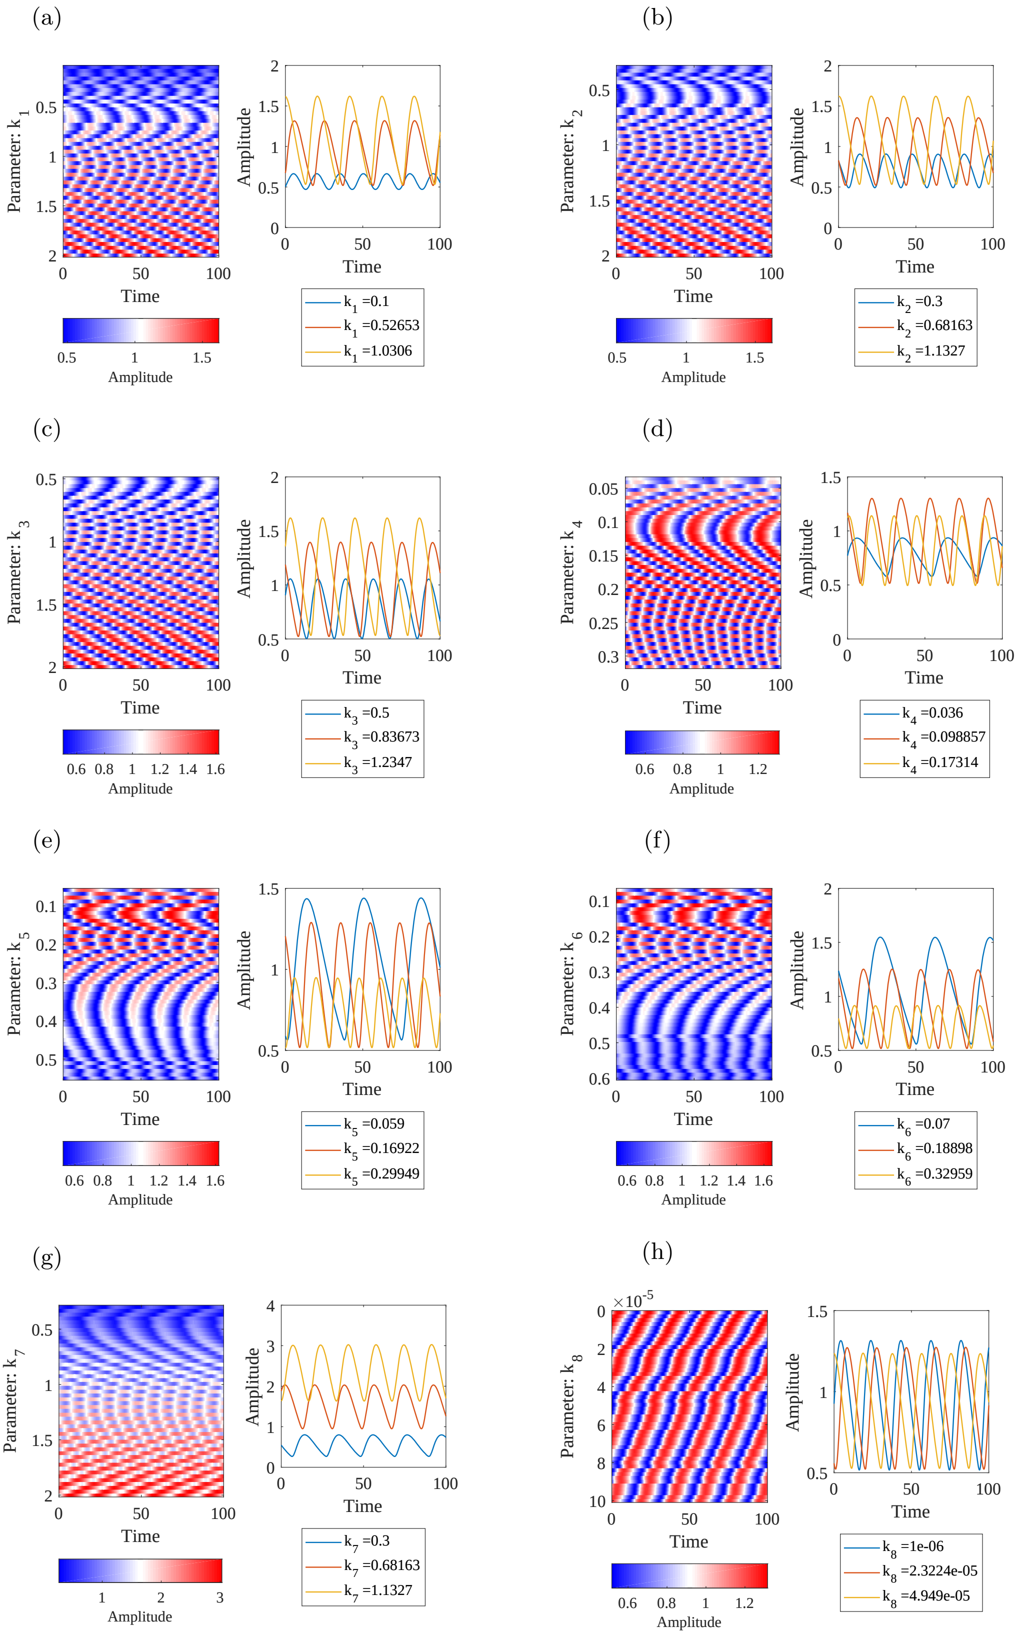


Figure 11-A : Kim-Forger model. a) (left) Color-map with $k_1 = 0.1$ to 2. (right) Trajectories for different values of $k_1$. b) (left) Color-map with $k_2 = 0.3$ to 2. (right) Trajectories for different values of $k_2$. c) (left) Color-map with $k_3 = 0.5$ to 2. (right) Trajectories for different values of $k_3$. d) (left) Color-map with $k_4 = 0.036$ to 0.316. (right) Trajectories for different values of $k_4$. e) (left) Color-map with $k_5 = 0.049$ to 0.579. (right) Trajectories for different values of $k_5$. f) (left) Color-map with $k_6 = 0.3$ to 0.6. (right) Trajectories for different values of $k_6$.g) (left) Color-map with $k_7 = 0.3$ to 2. (right) Trajectories for different values of $k_7$.h) (left) Color-map with $k_8 = 10^{-6}$ to $10^{-4}$. (right) Trajectories for different values of $k_8$.

## 11.2 Co-variation of period and maximum amplitude

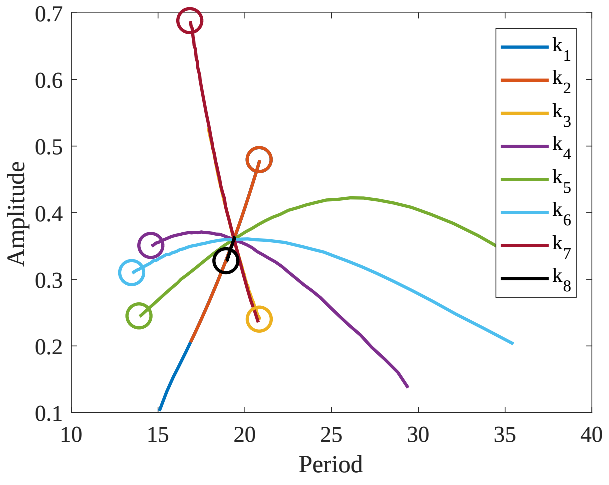


Figure 11-B : Kim-Forger model. Co-variation of period and maximum amplitude. Circle shaped markers represent the largest value of the corresponding parameter. As parameter $k_1$ increases, the amplitude increases and the period increases. As parameter $k_2$ increases, the amplitude increases and the period increases. As parameter $k_3$ increases, the amplitude decreases and the period does not change significantly. As parameter $k_4$ increases, the amplitude first increases then decreases and the period decreases. As parameter $k_5$ increases, the amplitude first increases then decreases and the period decreases. As parameter $k_6$ increases, the amplitude first increases then decreases and the period decreases. As parameter $k_7$ increases, the amplitude increases and the period decreases. As parameter $k_8$ increases, the amplitude and period does not change significantly.

## 11.3 Co-variation of period and amplitude metric ($M_p$)

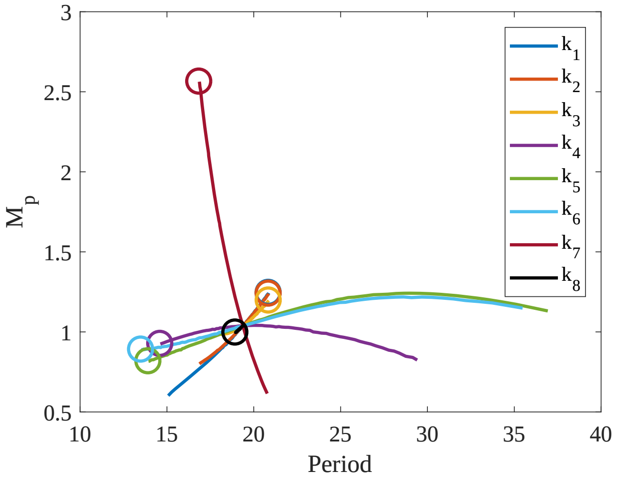


Figure 11-C : Kim-Forger model. Co-variation of period and amplitude metric ($M_p$). Circle shaped markers represent the largest value of the corresponding parameter. As parameters $k_1$, $k_2$ and $k_3$ increases, $M_p$ increases and the period increases. As parameter $k_4$ increases, $M_p$ first increases then decreases but the period decreases. As parameter $k_5$ increases, $M_p$ first increases then decreases but the period decreases. As parameter $k_6$ increases, $M_p$ first increases then decreases but the period decreases. As parameter $k_7$ increases, $M_p$ increases and period slightly decreases. As parameter $k_8$ increases, $M_p$ and period remains constant.

## References


[1] Elowitz, M.B., Leibler, S.: 'A synthetic oscillatory network of transcriptional regulators', *Nature*, 2000, **403**, (6767), pp. 335–338

[2] Tsai, T.Y.C., Choi, Y.S., Ma, W., Pomerening, J.R., Tang, C., Ferrell, J.E.: 'Robust, tunable biological oscillations from interlinked positive and negative feedback loops', *Science*, 2008, **321**, (5885), pp. 126–129

[3] Goodwin, B.C.: 'Oscillatory behavior in enzymatic control processes', *Advances in Enzyme Regulation*, 1965, **3**, pp. 425 – 437

[4] Pol, B.V.D.: 'The nonlinear theory of electric oscillations', *Proceedings of the Institute of Radio Engineers*, 1934, **22(9)**, pp. 1051–86

[5] FitzHugh, R.: 'Impulses and physiological states in theoretical models of nerve membrane', *Biophysical Journal*, 1961, **1(6)**, pp. 445–466

[6] Nagumo, J., Arimoto, S., Yoshizawa, S.: 'An active pulse transmission line simulating nerve axon', *Proceedings of the Institute of Radio Engineers*, 1962, **50**, pp. 2061–2070

[7] Igoshin, O.A., Goldbeter, A., Kaiser, D., Oster, G.: 'A biochemical oscillator explains several aspects of *Myxococcus xanthus* behavior during development', *Proceedings of the National Academy of Sciences of the United States of America*, 2004, **101**, (44), pp. 15760–15765

[8] Nakajima, M., Imai, K., Ito, H., Nishiwaki, T., Murayama, Y., Iwasaki, H., et al.: 'Reconstitution of circadian oscillation of cyanobacterial KaiC phosphorylation in vitro', *Science*, 2005, **308**, (5720), pp. 414–415

[9] Rust, M.J., Markson, J.S., Lane, W.S., Fisher, D.S., O'Shea, E.K.: 'Ordered phosphorylation governs oscillation of a three-protein circadian clock', *Science*, 2007, **318**, (5851), pp. 809–812

[10] Fung, E., Wong, W.W., Suen, J.K., Bulter, T., Lee, S.g., Liao, J.C.: 'A synthetic gene-metabolic oscillator', *Nature*, 2005, **435**, (7038), pp. 118–122

[11] Hasty, J., Dolnik, M., Rosttschafer, V., Collins, J.J.: 'Synthetic gene network for entraining and amplifying cellular oscillations', *The American Physical Society*, 2002, **88(14)**, pp. 148101–1–4

[12] Meyer, T., Stryer, L.: 'Molecular model for receptor-stimulated calcium spiking', *Proceedings of the National Academy of Sciences of the United States of America*, 1988, **85**, (14), pp. 5051–5055

[13] Kim, J.K.: 'Protein sequestration versus hill-type repression in circadian clock models', *IET Systems Biology*, 2016, **10**, pp. 125–135(10)
